# Supplementary material for: The Apollonian structure of integer superharmonic matrices
Source: arXiv:1309.3267 ancillary file (2017-07-17)

# EXTENDED APPENDIX TO: THE APOLLONIAN STRUCTURE OF INTEGER SUPERHARMONIC MATRICES

LIONEL LEVINE, WESLEY PEGDEN, AND CHARLES K. SMART

Here we display proper Descartes quadruples $(C_0, C_1, C_2, C_3) \in \mathcal{B}$, along with the Soddy precursor $C_4 = 2(C_1 + C_2 + C_3) - C_0$ of $C_0$, the vectors $v(C_i, C_0)$ and $a(C_i, C_0)$ $(i = 1, 2, 3)$, the tile odometer for $C_0$, and a tiling neighborhood in $T_C + L_C$. We display quadruples up to symmetry for $1 \le c_0 \le 500$.

| $C_0$<br>$C_1$<br>$C_2$<br>$C_3$<br>$C_4$ | <br>$v(C_1,C_0)$<br>$v(C_2,C_0)$<br>$v(C_3,C_0)$ | <br>$a(C_1,C_0)$<br>$a(C_2,C_0)$<br>$a(C_3,C_0)$ | tile odometer | One neighborhood of $T_C$ in $T_C + L_C$. |
|---|---|---|---|---|
| $(4, 1+4i)$ | | | 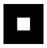 | 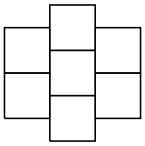 |
| $(1, 1+2i)$ | $2+1i$ | $1+1i$ | | |
| $(1, 1)$ | $-2+1i$ | $-1i$ | | |
| $(0, -1)$ | $-2i$ | $-1$ | | |
| $(0, 1)$ | | | | |
| $(9, 1+6i)$ | | | 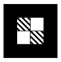 | 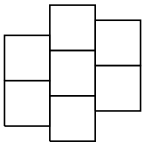 |
| $(4, 1+4i)$ | $3+2i$ | $1+1i$ | | |
| $(1, 1)$ | $-3+1i$ | $-1i$ | | |
| $(0, -1)$ | $-3i$ | $-1$ | | |
| $(1, 1+2i)$ | | | | |
| $(12, 7+12i)$ | | | 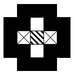 | 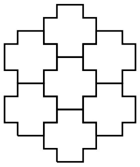 |
| $(4, 1+4i)$ | $-4i$ | $-2+1i$ | | |
| $(1, 1+2i)$ | $3+2i$ | $2+1i$ | | |
| $(1, 1)$ | $-3+2i$ | $-2i$ | | |
| $(0, -1)$ | | | | |
| $(16, 1+8i)$ | | | 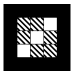 | 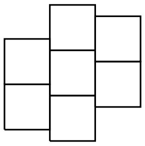 |
| $(9, 1+6i)$ | $4+3i$ | $1+1i$ | | |
| $(1, 1)$ | $-4+1i$ | $-1i$ | | |
| $(0, -1)$ | $-4i$ | $-1$ | | |
| $(4, 1+4i)$ | | | | |
| $(24, 17+24i)$ | | | 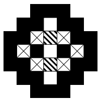 | 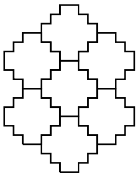 |
| $(12, 7+12i)$ | $-6i$ | $-3+2i$ | | |
| $(1, 1+2i)$ | $4+3i$ | $3+1i$ | | |
| $(1, 1)$ | $-4+3i$ | $-3i$ | | |
| $(4, 1+4i)$ | | | | |
| $(25, 1+10i)$ | | | 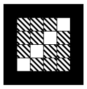 | 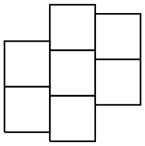 |
| $(16, 1+8i)$ | $5+4i$ | $1+1i$ | | |
| $(1, 1)$ | $-5+1i$ | $-1i$ | | |
| $(0, -1)$ | $-5i$ | $-1$ | | |
| $(9, 1+6i)$ | | | | |
| $(25, 1+20i)$ | | | 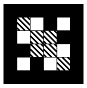 | 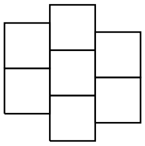 |
| $(9, 1+6i)$ | $-5+3i$ | $1-2i$ | | |
| $(0, -1)$ | $-5i$ | $-2$ | | |
| $(4, 1+4i)$ | $5+2i$ | $1+2i$ | | |
| $(1, 1)$ | | | | |

*Date*: May 22, 2014.

| | | |
|---|---|---|
| $(28, 7+20i)$ | | |
| $(9, 1+6i)$ | $1-6i$ | $-2+1i$ |
| $(4, 1+4i)$ | $4+4i$ | $2+1i$ |
| $(1, 1)$ | $-5+2i$ | $-2i$ |
| $(0, -1)$ | | |

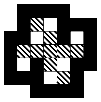
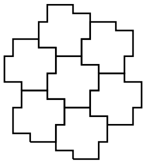

| | | |
|---|---|---|
| $(33, 17+30i)$ | | |
| $(12, 7+12i)$ | $6+3i$ | $3+2i$ |
| $(1, 1)$ | $-5+3i$ | $-3i$ |
| $(4, 1+4i)$ | $-1-6i$ | $-3+1i$ |
| $(1, 1+2i)$ | | |

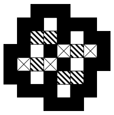
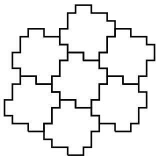

| | | |
|---|---|---|
| $(36, 1+12i)$ | | |
| $(25, 1+10i)$ | $6+5i$ | $1+1i$ |
| $(1, 1)$ | $-6+1i$ | $-1i$ |
| $(0, -1)$ | $-6i$ | $-1$ |
| $(16, 1+8i)$ | | |

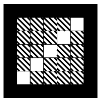
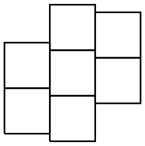

| | | |
|---|---|---|
| $(40, 31+40i)$ | | |
| $(24, 17+24i)$ | $-8i$ | $-4+3i$ |
| $(1, 1+2i)$ | $5+4i$ | $4+1i$ |
| $(1, 1)$ | $-5+4i$ | $-4i$ |
| $(12, 7+12i)$ | | |

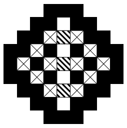
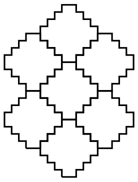

| | | |
|---|---|---|
| $(49, 1+14i)$ | | |
| $(36, 1+12i)$ | $7+6i$ | $1+1i$ |
| $(1, 1)$ | $-7+1i$ | $-1i$ |
| $(0, -1)$ | $-7i$ | $-1$ |
| $(25, 1+10i)$ | | |

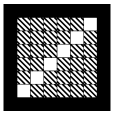
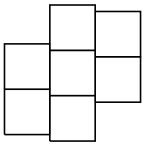

| | | |
|---|---|---|
| $(49, 1+28i)$ | | |
| $(16, 1+8i)$ | $-7+4i$ | $1-2i$ |
| $(0, -1)$ | $-7i$ | $-2$ |
| $(9, 1+6i)$ | $7+3i$ | $1+2i$ |
| $(1, 1)$ | | |

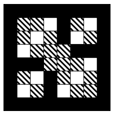
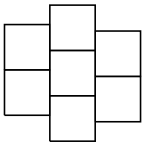

| | | |
|---|---|---|
| $(49, 1+42i)$ | | |
| $(25, 1+20i)$ | $-7+5i$ | $2-3i$ |
| $(0, -1)$ | $-7i$ | $-3$ |
| $(4, 1+4i)$ | $7+2i$ | $1+3i$ |
| $(9, 1+6i)$ | | |

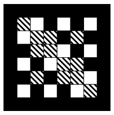
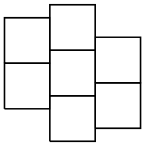

| | | |
|---|---|---|
| $(52, 7+28i)$ | | |
| $(16, 1+8i)$ | $2-8i$ | $-2+1i$ |
| $(9, 1+6i)$ | $5+6i$ | $2+1i$ |
| $(1, 1)$ | $-7+2i$ | $-2i$ |
| $(0, -1)$ | | |

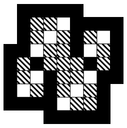
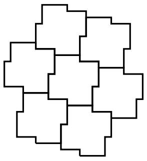

| | | |
|---|---|---|
| $(57, 17+42i)$ | | |
| $(28, 7+20i)$ | $2-9i$ | $-3+2i$ |
| $(4, 1+4i)$ | $5+6i$ | $3+1i$ |
| $(1, 1)$ | $-7+3i$ | $-3i$ |
| $(9, 1+6i)$ | | |

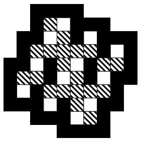
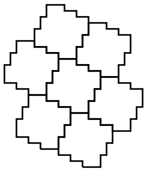

| | | |
|---|---|---|
| $(60, 49+60i)$ | | |
| $(40, 31+40i)$ | $-10i$ | $-5+4i$ |
| $(1, 1+2i)$ | $6+5i$ | $5+1i$ |
| $(1, 1)$ | $-6+5i$ | $-5i$ |
| $(24, 17+24i)$ | | |

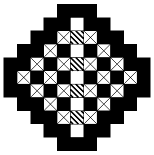
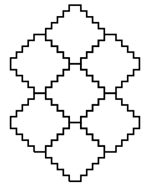

| | | |
|---|---|---|
| $(64, 1+16i)$ | | |
| $(49, 1+14i)$ | $8+7i$ | $1+1i$ |
| $(1, 1)$ | $-8+1i$ | $-1i$ |
| $(0, -1)$ | $-8i$ | $-1$ |
| $(36, 1+12i)$ | | |

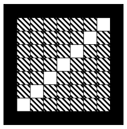
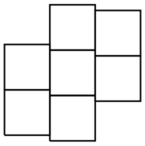

| | | |
|---|---|---|
| $(64, 1+48i)$ | | |
| $(25, 1+20i)$ | $8+5i$ | $2+3i$ |
| $(9, 1+6i)$ | $-8+3i$ | $1-3i$ |
| $(0, -1)$ | $-8i$ | $-3$ |
| $(4, 1+4i)$ | | |

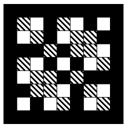
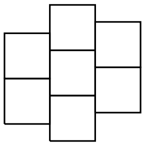

| | | |
|---|---|---|
| $(64, 31+56i)$ | | |
| $(33, 17+30i)$ | $9+4i$ | $4+3i$ |
| $(1, 1)$ | $-7+4i$ | $-4i$ |
| $(4, 1+4i)$ | $-2-8i$ | $-4+1i$ |
| $(12, 7+12i)$ | | |

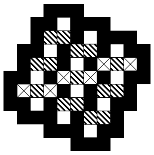
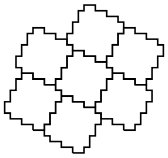

| | | |
|---|---|---|
| $(72, 17+48i)$ | | |
| $(28, 7+20i)$ | $8+6i$ | $3+2i$ |
| $(1, 1)$ | $-8+3i$ | $-3i$ |
| $(9, 1+6i)$ | $-9i$ | $-3+1i$ |
| $(4, 1+4i)$ | | |

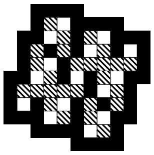
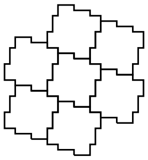

| | | |
|---|---|---|
| $(73, 49+70i)$ | | |
| $(24, 17+24i)$ | $9+4i$ | $5+3i$ |
| $(1, 1)$ | $-7+5i$ | $-5i$ |
| $(12, 7+12i)$ | $-2-9i$ | $-5+2i$ |
| $(1, 1+2i)$ | | |

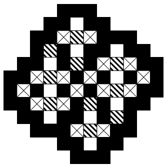
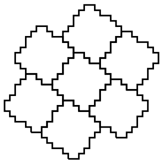

| | | |
|---|---|---|
| $(76, 7+60i)$ | | |
| $(25, 1+20i)$ | $-1-10i$ | $-4$ |
| $(4, 1+4i)$ | $8+4i$ | $2+3i$ |
| $(9, 1+6i)$ | $-7+6i$ | $2-3i$ |
| $(0, -1)$ | | |

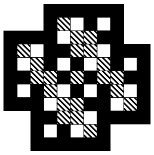
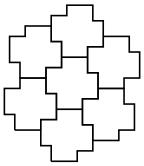

| | | |
|---|---|---|
| $(81, 1+18i)$ | | |
| $(64, 1+16i)$ | $9+8i$ | $1+1i$ |
| $(1, 1)$ | $-9+1i$ | $-1i$ |
| $(0, -1)$ | $-9i$ | $-1$ |
| $(49, 1+14i)$ | | |

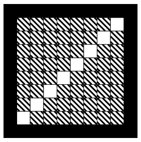
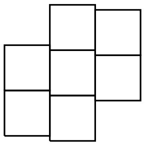

| | | |
|---|---|---|
| $(81, 1+36i)$ | | |
| $(25, 1+10i)$ | $-9+5i$ | $1-2i$ |
| $(0, -1)$ | $-9i$ | $-2$ |
| $(16, 1+8i)$ | $9+4i$ | $1+2i$ |
| $(1, 1)$ | | |

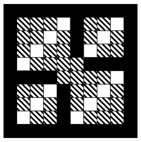
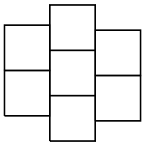

| | | |
|---|---|---|
| $(81, 17+60i)$ | | |
| $(28, 7+20i)$ | $-10+3i$ | $-4i$ |
| $(9, 1+6i)$ | $3-9i$ | $-3+2i$ |
| $(4, 1+4i)$ | $7+6i$ | $3+2i$ |
| $(1, 1)$ | | |

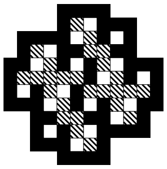
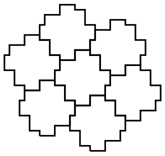

| | | |
|---|---|---|
| $(81, 1+72i)$ | | |
| $(49, 1+42i)$ | $-9+7i$ | $3-4i$ |
| $(0, -1)$ | $-9i$ | $-4$ |
| $(4, 1+4i)$ | $9+2i$ | $1+4i$ |
| $(25, 1+20i)$ | | |

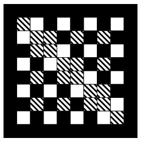
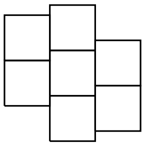

| | | |
|---|---|---|
| $(84, 7+36i)$ | | |
| $(25, 1+10i)$ | $3-10i$ | $-2+1i$ |
| $(16, 1+8i)$ | $6+8i$ | $2+1i$ |
| $(1, 1)$ | $-9+2i$ | $-2i$ |
| $(0, -1)$ | | |

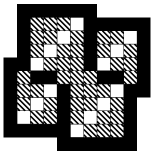
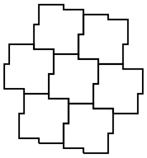

| | | |
|---|---|---|
| $(84, 71+84i)$ | | |
| $(60, 49+60i)$ | $-12i$ | $-6+5i$ |
| $(1, 1+2i)$ | $7+6i$ | $6+1i$ |
| $(1, 1)$ | $-7+6i$ | $-6i$ |
| $(40, 31+40i)$ | | |

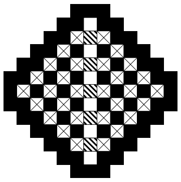
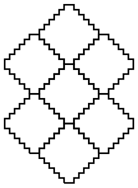

| | | |
|---|---|---|
| $(88, 49+80i)$ | | |
| $(33, 17+30i)$ | $-11i$ | $-5+3i$ |
| $(12, 7+12i)$ | $8+6i$ | $5+2i$ |
| $(1, 1)$ | $-8+5i$ | $-5i$ |
| $(4, 1+4i)$ | | |

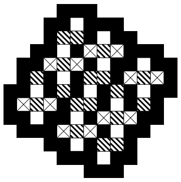
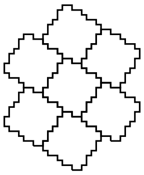

| | | |
|---|---|---|
| $(96, 31+72i)$ | | |
| $(57, 17+42i)$ | $3-12i$ | $-4+3i$ |
| $(4, 1+4i)$ | $6+8i$ | $4+1i$ |
| $(1, 1)$ | $-9+4i$ | $-4i$ |
| $(28, 7+20i)$ | | |

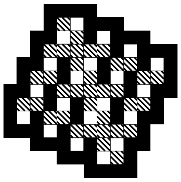
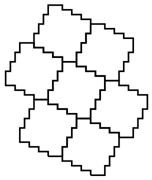

| | | |
|---|---|---|
| $(97, 49+92i)$ | | |
| $(33, 17+30i)$ | $-9+7i$ | $1-6i$ |
| $(4, 1+4i)$ | $-1-10i$ | $-5+2i$ |
| $(12, 7+12i)$ | $10+3i$ | $4+4i$ |
| $(1, 1)$ | | |

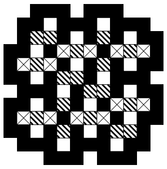
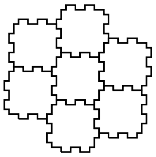

| | | |
|---|---|---|
| $(100, 1+20i)$ | | |
| $(81, 1+18i)$ | $10+9i$ | $1+1i$ |
| $(1, 1)$ | $-10+1i$ | $-1i$ |
| $(0, -1)$ | $-10i$ | $-1$ |
| $(64, 1+16i)$ | | |

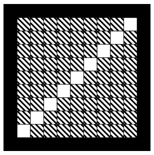
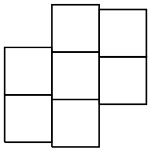

| | | |
|---|---|---|
| $(100, 1+60i)$ | | |
| $(49, 1+28i)$ | $-10+7i$ | $2-3i$ |
| $(0, -1)$ | $-10i$ | $-3$ |
| $(9, 1+6i)$ | $10+3i$ | $1+3i$ |
| $(16, 1+8i)$ | | |

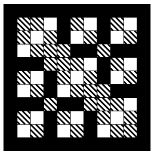
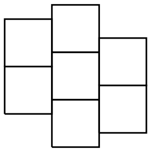

| | | |
|---|---|---|
| $(105, 49+90i)$ | | |
| $(64, 31+56i)$ | $12+5i$ | $5+4i$ |
| $(1, 1)$ | $-9+5i$ | $-5i$ |
| $(4, 1+4i)$ | $-3-10i$ | $-5+1i$ |
| $(33, 17+30i)$ | | |

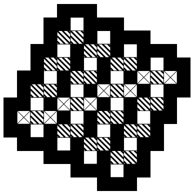
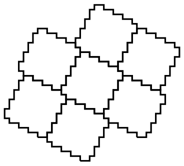

| | | |
|---|---|---|
| $(108, 17+60i)$ | | |
| $(52, 7+28i)$ | $4-12i$ | $-3+2i$ |
| $(9, 1+6i)$ | $6+9i$ | $3+1i$ |
| $(1, 1)$ | $-10+3i$ | $-3i$ |
| $(16, 1+8i)$ | | |

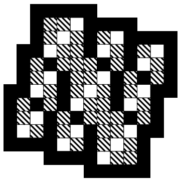
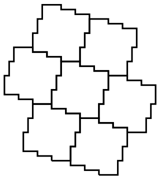

| | | |
|---|---|---|
| $(112, 97+112i)$ | | |
| $(84, 71+84i)$ | $-14i$ | $-7+6i$ |
| $(1, 1+2i)$ | $8+7i$ | $7+1i$ |
| $(1, 1)$ | $-8+7i$ | $-7i$ |
| $(60, 49+60i)$ | | |

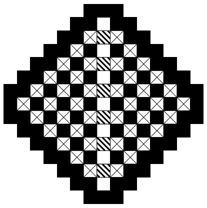
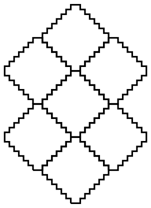

| | | |
|---|---|---|
| $(121, 1+22i)$ | | |
| $(100, 1+20i)$ | $11+10i$ | $1+1i$ |
| $(1,1)$ | $-11+1i$ | $-1i$ |
| $(0,-1)$ | $-11i$ | $-1$ |
| $(81, 1+18i)$ | | |

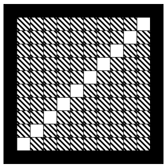
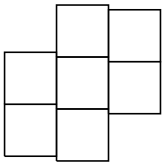

| | | |
|---|---|---|
| $(121, 1+44i)$ | | |
| $(36, 1+12i)$ | $-11+6i$ | $1-2i$ |
| $(0,-1)$ | $-11i$ | $-2$ |
| $(25, 1+10i)$ | $11+5i$ | $1+2i$ |
| $(1,1)$ | | |

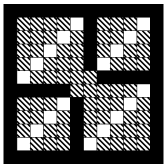
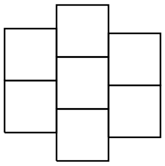

| | | |
|---|---|---|
| $(121, 1+66i)$ | | |
| $(49, 1+28i)$ | $11+7i$ | $2+3i$ |
| $(16, 1+8i)$ | $-11+4i$ | $1-3i$ |
| $(0,-1)$ | $-11i$ | $-3$ |
| $(9, 1+6i)$ | | |

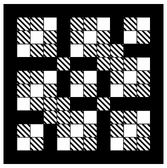
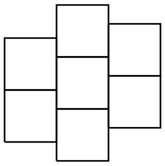

| | | |
|---|---|---|
| $(121, 1+88i)$ | | |
| $(64, 1+48i)$ | $11+8i$ | $3+4i$ |
| $(9, 1+6i)$ | $-11+3i$ | $1-4i$ |
| $(0,-1)$ | $-11i$ | $-4$ |
| $(25, 1+20i)$ | | |

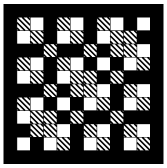
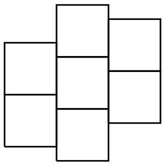

| | | |
|---|---|---|
| $(121, 1+110i)$ | | |
| $(81, 1+72i)$ | $-11+9i$ | $4-5i$ |
| $(0,-1)$ | $-11i$ | $-5$ |
| $(4, 1+4i)$ | $11+2i$ | $1+5i$ |
| $(49, 1+42i)$ | | |

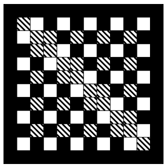
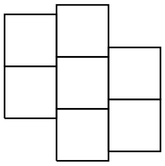

| | | |
|---|---|---|
| $(124, 7+44i)$ | | |
| $(36, 1+12i)$ | $4-12i$ | $-2+1i$ |
| $(25, 1+10i)$ | $7+10i$ | $2+1i$ |
| $(1,1)$ | $-11+2i$ | $-2i$ |
| $(0,-1)$ | | |

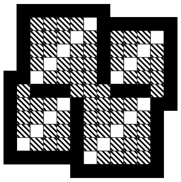
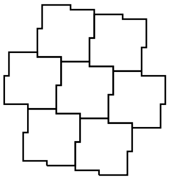

| | | |
|---|---|---|
| $(129, 17+66i)$ | | |
| $(52, 7+28i)$ | $10+9i$ | $3+2i$ |
| $(1,1)$ | $-11+3i$ | $-3i$ |
| $(16, 1+8i)$ | $1-12i$ | $-3+1i$ |
| $(9, 1+6i)$ | | |

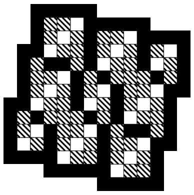
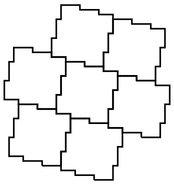

| | | |
|---|---|---|
| $(129, 97+126i)$ | | |
| $(40, 31+40i)$ | $12+5i$ | $7+4i$ |
| $(1,1)$ | $-9+7i$ | $-7i$ |
| $(24, 17+24i)$ | $-3-12i$ | $-7+3i$ |
| $(1, 1+2i)$ | | |

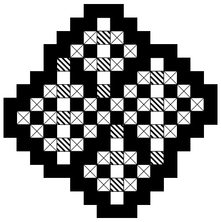
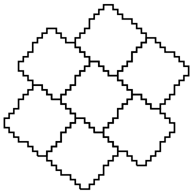

| | | |
|---|---|---|
| $(136, 31+88i)$ | | |
| $(72, 17+48i)$ | $12+8i$ | $4+3i$ |
| $(1,1)$ | $-11+4i$ | $-4i$ |
| $(9, 1+6i)$ | $-1-12i$ | $-4+1i$ |
| $(28, 7+20i)$ | | |

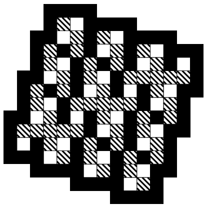
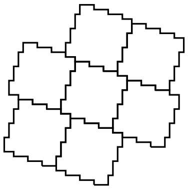

| | | |
|---|---|---|
| $(144, 1+24i)$ | | |
| $(121, 1+22i)$ | $12+11i$ | $1+1i$ |
| $(1, 1)$ | $-12+1i$ | $-1i$ |
| $(0, -1)$ | $-12i$ | $-1$ |
| $(100, 1+20i)$ | | |

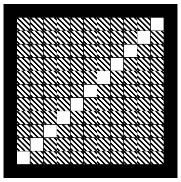
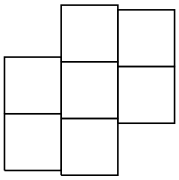

| | | |
|---|---|---|
| $(144, 1+120i)$ | | |
| $(49, 1+42i)$ | $12+7i$ | $3+5i$ |
| $(25, 1+20i)$ | $-12+5i$ | $2-5i$ |
| $(0, -1)$ | $-12i$ | $-5$ |
| $(4, 1+4i)$ | | |

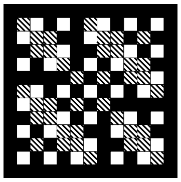
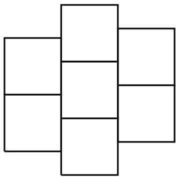

| | | |
|---|---|---|
| $(144, 127+144i)$ | | |
| $(112, 97+112i)$ | $-16i$ | $-8+7i$ |
| $(1, 1+2i)$ | $9+8i$ | $8+1i$ |
| $(1, 1)$ | $-9+8i$ | $-8i$ |
| $(84, 71+84i)$ | | |

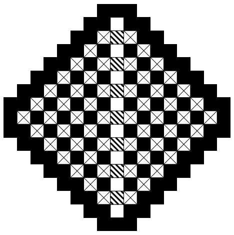
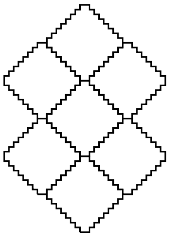

| | | |
|---|---|---|
| $(145, 49+110i)$ | | |
| $(96, 31+72i)$ | $4-15i$ | $-5+4i$ |
| $(4, 1+4i)$ | $7+10i$ | $5+1i$ |
| $(1, 1)$ | $-11+5i$ | $-5i$ |
| $(57, 17+42i)$ | | |

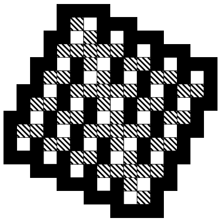
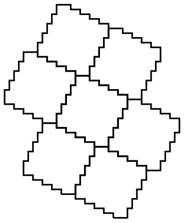

| | | |
|---|---|---|
| $(148, 7+84i)$ | | |
| $(49, 1+28i)$ | $-1-14i$ | $-4$ |
| $(9, 1+6i)$ | $11+6i$ | $2+3i$ |
| $(16, 1+8i)$ | $-10+8i$ | $2-3i$ |
| $(0, -1)$ | | |

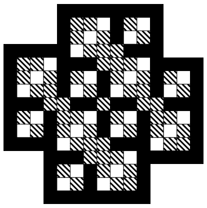
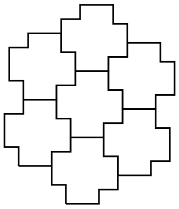

| | | |
|---|---|---|
| $(148, 97+140i)$ | | |
| $(73, 49+70i)$ | $14+5i$ | $7+5i$ |
| $(1, 1)$ | $-10+7i$ | $-7i$ |
| $(12, 7+12i)$ | $-4-12i$ | $-7+2i$ |
| $(24, 17+24i)$ | | |

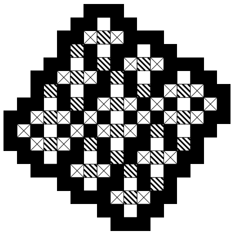
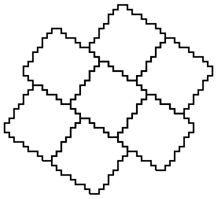

| | | |
|---|---|---|
| $(153, 17+84i)$ | | |
| $(52, 7+28i)$ | $-14+3i$ | $-4i$ |
| $(16, 1+8i)$ | $5-12i$ | $-3+2i$ |
| $(9, 1+6i)$ | $9+9i$ | $3+2i$ |
| $(1, 1)$ | | |

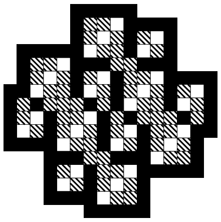
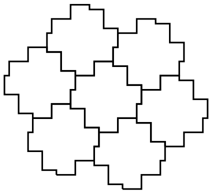

| | | |
|---|---|---|
| $(153, 17+120i)$ | | |
| $(76, 7+60i)$ | $-2-15i$ | $-6$ |
| $(4, 1+4i)$ | $11+6i$ | $3+4i$ |
| $(9, 1+6i)$ | $-9+9i$ | $3-4i$ |
| $(25, 1+20i)$ | | |

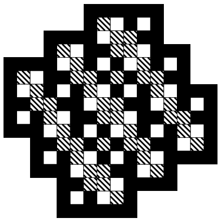
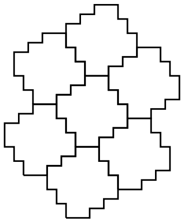

| | | |
|---|---|---|
| $(156, 7+132i)$ | | |
| $(49, 1+42i)$ | $-3-14i$ | $-6-1i$ |
| $(4, 1+4i)$ | $12+4i$ | $2+5i$ |
| $(25, 1+20i)$ | $-9+10i$ | $4-4i$ |
| $(0, -1)$ | | |

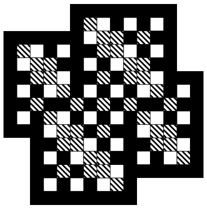
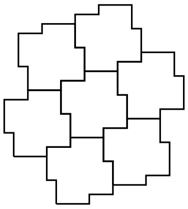

| | | |
|---|---|---|
| $(156, 71+132i)$ | | |
| $(105, 49+90i)$ | $15+6i$ | $6+5i$ |
| $(1, 1)$ | $-11+6i$ | $-6i$ |
| $(4, 1+4i)$ | $-4-12i$ | $-6+1i$ |
| $(64, 31+56i)$ | | |

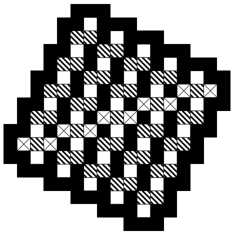
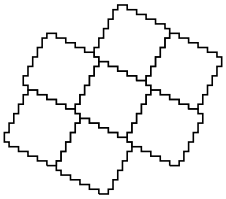

| | | |
|---|---|---|
| $(160, 31+120i)$ | | |
| $(81, 17+60i)$ | $-15+4i$ | $-6i$ |
| $(9, 1+6i)$ | $5-12i$ | $-4+3i$ |
| $(4, 1+4i)$ | $10+8i$ | $4+3i$ |
| $(28, 7+20i)$ | | |

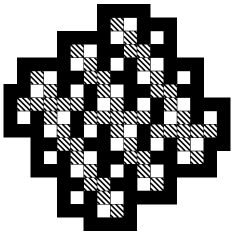
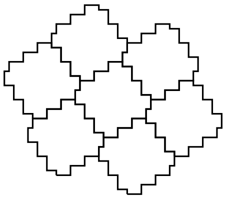

| | | |
|---|---|---|
| $(168, 49+120i)$ | | |
| $(57, 17+42i)$ | $12+9i$ | $5+3i$ |
| $(1, 1)$ | $-12+5i$ | $-5i$ |
| $(28, 7+20i)$ | $-14i$ | $-5+2i$ |
| $(4, 1+4i)$ | | |

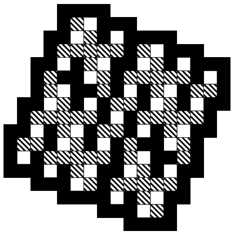
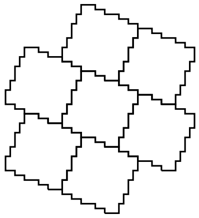

| | | |
|---|---|---|
| $(169, 1+26i)$ | | |
| $(144, 1+24i)$ | $13+12i$ | $1+1i$ |
| $(1, 1)$ | $-13+1i$ | $-1i$ |
| $(0, -1)$ | $-13i$ | $-1$ |
| $(121, 1+22i)$ | | |

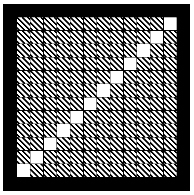
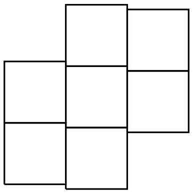

| | | |
|---|---|---|
| $(169, 1+52i)$ | | |
| $(49, 1+14i)$ | $-13+7i$ | $1-2i$ |
| $(0, -1)$ | $-13i$ | $-2$ |
| $(36, 1+12i)$ | $13+6i$ | $1+2i$ |
| $(1, 1)$ | | |

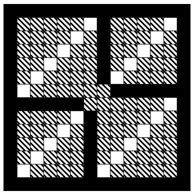
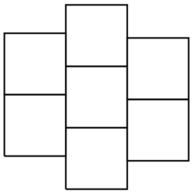

| | | |
|---|---|---|
| $(169, 1+78i)$ | | |
| $(81, 1+36i)$ | $-13+9i$ | $2-3i$ |
| $(0, -1)$ | $-13i$ | $-3$ |
| $(16, 1+8i)$ | $13+4i$ | $1+3i$ |
| $(25, 1+10i)$ | | |

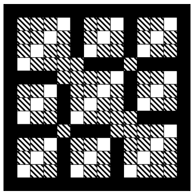
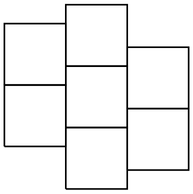

| | | |
|---|---|---|
| $(169, 1+104i)$ | | |
| $(100, 1+60i)$ | $-13+10i$ | $3-4i$ |
| $(0, -1)$ | $-13i$ | $-4$ |
| $(9, 1+6i)$ | $13+3i$ | $1+4i$ |
| $(49, 1+28i)$ | | |

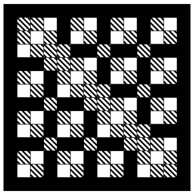
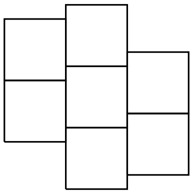

| | | |
|---|---|---|
| $(169, 1+130i)$ | | |
| $(64, 1+48i)$ | $-13+8i$ | $3-5i$ |
| $(0, -1)$ | $-13i$ | $-5$ |
| $(25, 1+20i)$ | $13+5i$ | $2+5i$ |
| $(9, 1+6i)$ | | |

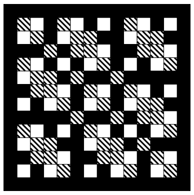
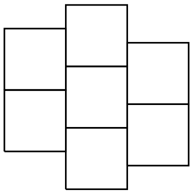

| | | |
|---|---|---|
| $(169, 1+156i)$ | | |
| $(121, 1+110i)$ | $-13+11i$ | $5-6i$ |
| $(0, -1)$ | $-13i$ | $-6$ |
| $(4, 1+4i)$ | $13+2i$ | $1+6i$ |
| $(81, 1+72i)$ | | |

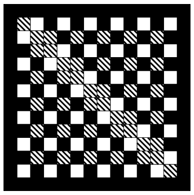
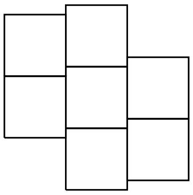

| | | |
|---|---|---|
| $(169, 97+154i)$ | | |
| $(88, 49+80i)$ | $1-16i$ | $-7+5i$ |
| $(12, 7+12i)$ | $10+9i$ | $7+2i$ |
| $(1, 1)$ | $-11+7i$ | $-7i$ |
| $(33, 17+30i)$ | | |

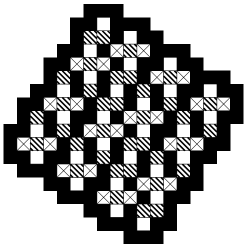
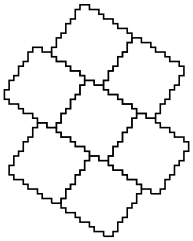

| | | |
|---|---|---|
| $(172, 7+52i)$ | | |
| $(49, 1+14i)$ | $5-14i$ | $-2+1i$ |
| $(36, 1+12i)$ | $8+12i$ | $2+1i$ |
| $(1, 1)$ | $-13+2i$ | $-2i$ |
| $(0, -1)$ | | |

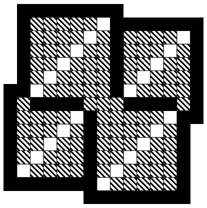
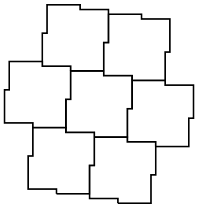

| | | |
|---|---|---|
| $(177, 17+78i)$ | | |
| $(84, 7+36i)$ | $6-15i$ | $-3+2i$ |
| $(16, 1+8i)$ | $7+12i$ | $3+1i$ |
| $(1, 1)$ | $-13+3i$ | $-3i$ |
| $(25, 1+10i)$ | | |

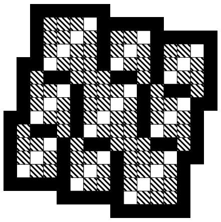
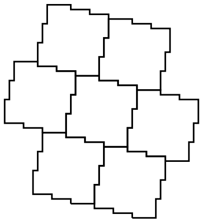

| | | |
|---|---|---|
| $(177, 49+132i)$ | | |
| $(57, 17+42i)$ | $-15+3i$ | $-1-6i$ |
| $(28, 7+20i)$ | $6-13i$ | $-4+4i$ |
| $(4, 1+4i)$ | $9+10i$ | $5+2i$ |
| $(1, 1)$ | | |

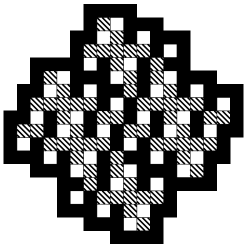
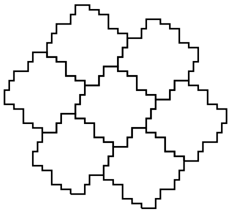

| | | |
|---|---|---|
| $(180, 161 + 180i)$ | | |
| $(144, 127 + 144i)$ | $-18i$ | $-9 + 8i$ |
| $(1, 1 + 2i)$ | $10 + 9i$ | $9 + 1i$ |
| $(1, 1)$ | $-10 + 9i$ | $-9i$ |
| $(112, 97 + 112i)$ | | |

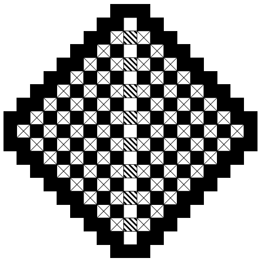
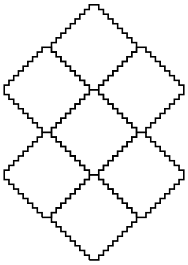

| | | |
|---|---|---|
| $(184, 31 + 104i)$ | | |
| $(108, 17 + 60i)$ | $6 - 16i$ | $-4 + 3i$ |
| $(9, 1 + 6i)$ | $7 + 12i$ | $4 + 1i$ |
| $(1, 1)$ | $-13 + 4i$ | $-4i$ |
| $(52, 7 + 28i)$ | | |

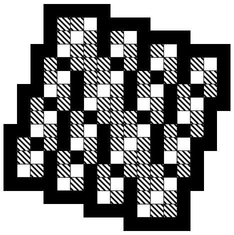
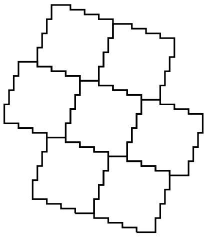

| | | |
|---|---|---|
| $(184, 127 + 176i)$ | | |
| $(73, 49 + 70i)$ | $-1 - 16i$ | $-8 + 5i$ |
| $(24, 17 + 24i)$ | $12 + 8i$ | $8 + 3i$ |
| $(1, 1)$ | $-11 + 8i$ | $-8i$ |
| $(12, 7 + 12i)$ | | |

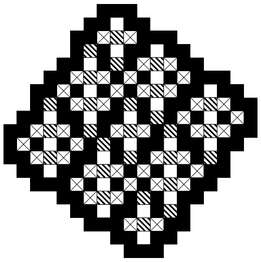
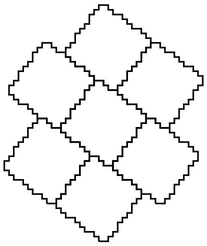

| | | |
|---|---|---|
| $(192, 97 + 168i)$ | | |
| $(64, 31 + 56i)$ | $-16i$ | $-7 + 4i$ |
| $(33, 17 + 30i)$ | $12 + 9i$ | $7 + 3i$ |
| $(1, 1)$ | $-12 + 7i$ | $-7i$ |
| $(4, 1 + 4i)$ | | |

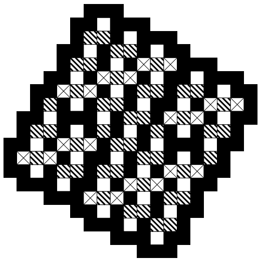
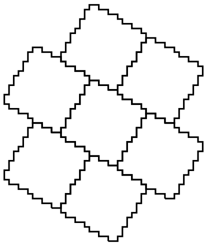

| | | |
|---|---|---|
| $(193, 49 + 130i)$ | | |
| $(72, 17 + 48i)$ | $3 - 16i$ | $-5 + 3i$ |
| $(28, 7 + 20i)$ | $10 + 11i$ | $5 + 2i$ |
| $(1, 1)$ | $-13 + 5i$ | $-5i$ |
| $(9, 1 + 6i)$ | | |

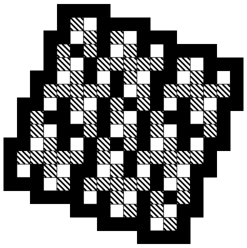
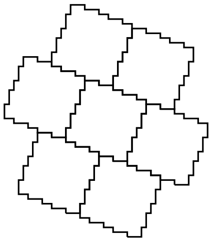

| | | |
|---|---|---|
| $(193, 97 + 186i)$ | | |
| $(97, 49 + 92i)$ | $-13 + 11i$ | $2 - 9i$ |
| $(4, 1 + 4i)$ | $-1 - 14i$ | $-7 + 3i$ |
| $(12, 7 + 12i)$ | $14 + 3i$ | $5 + 6i$ |
| $(33, 17 + 30i)$ | | |

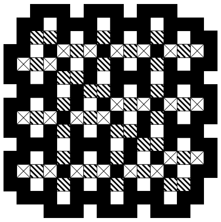
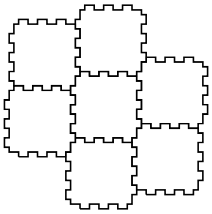

| | | |
|---|---|---|
| $(196, 1 + 28i)$ | | |
| $(169, 1 + 26i)$ | $14 + 13i$ | $1 + 1i$ |
| $(1, 1)$ | $-14 + 1i$ | $-1i$ |
| $(0, -1)$ | $-14i$ | $-1$ |
| $(144, 1 + 24i)$ | | |

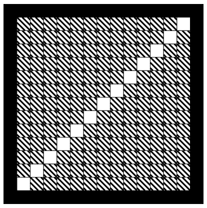
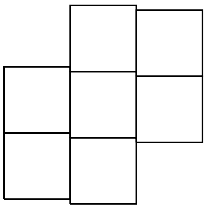

| | | |
|---|---|---|
| $(196, 1+84i)$ | | |
| $(81, 1+36i)$ | $14+9i$ | $2+3i$ |
| $(25, 1+10i)$ | $-14+5i$ | $1-3i$ |
| $(0, -1)$ | $-14i$ | $-3$ |
| $(16, 1+8i)$ | | |

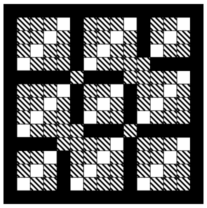
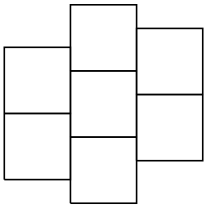

| | | |
|---|---|---|
| $(196, 1+140i)$ | | |
| $(121, 1+88i)$ | $14+11i$ | $4+5i$ |
| $(9, 1+6i)$ | $-14+3i$ | $1-5i$ |
| $(0, -1)$ | $-14i$ | $-5$ |
| $(64, 1+48i)$ | | |

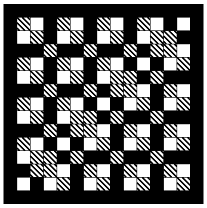
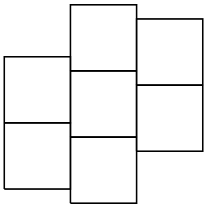

| | | |
|---|---|---|
| $(196, 7+148i)$ | | |
| $(64, 1+48i)$ | $2-16i$ | $-6+1i$ |
| $(25, 1+20i)$ | $11+10i$ | $4+4i$ |
| $(9, 1+6i)$ | $-13+6i$ | $2-5i$ |
| $(0, -1)$ | | |

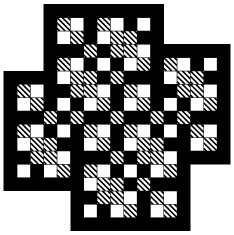
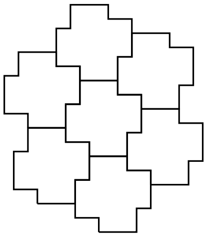

| | | |
|---|---|---|
| $(201, 17+162i)$ | | |
| $(76, 7+60i)$ | $-14+9i$ | $3-6i$ |
| $(25, 1+20i)$ | $1-15i$ | $-6+1i$ |
| $(4, 1+4i)$ | $13+6i$ | $3+5i$ |
| $(9, 1+6i)$ | | |

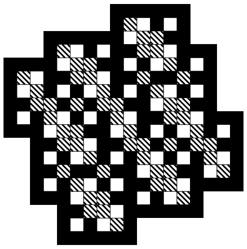
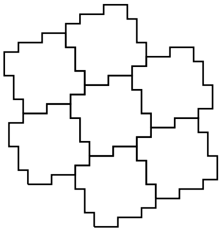

| | | |
|---|---|---|
| $(201, 97+180i)$ | | |
| $(64, 31+56i)$ | $-12+11i$ | $2-8i$ |
| $(4, 1+4i)$ | $-3-14i$ | $-7+2i$ |
| $(33, 17+30i)$ | $15+3i$ | $5+6i$ |
| $(1, 1)$ | | |

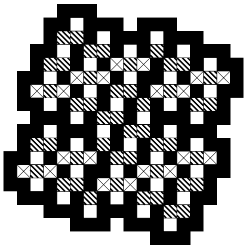
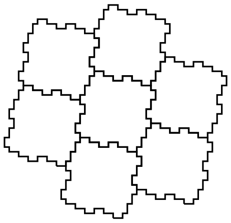

| | | |
|---|---|---|
| $(201, 161+198i)$ | | |
| $(60, 49+60i)$ | $15+6i$ | $9+5i$ |
| $(1, 1)$ | $-11+9i$ | $-9i$ |
| $(40, 31+40i)$ | $-4-15i$ | $-9+4i$ |
| $(1, 1+2i)$ | | |

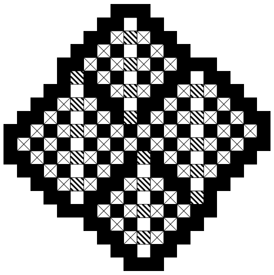
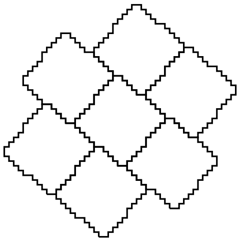

| | | |
|---|---|---|
| $(204, 17+84i)$ | | |
| $(84, 7+36i)$ | $12+12i$ | $3+2i$ |
| $(1, 1)$ | $-14+3i$ | $-3i$ |
| $(25, 1+10i)$ | $2-15i$ | $-3+1i$ |
| $(16, 1+8i)$ | | |

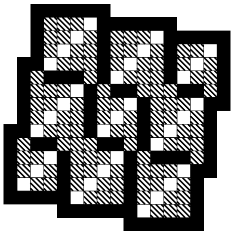
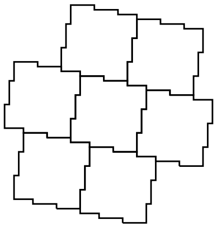

| | | |
|---|---|---|
| $(204, 71+156i)$ | | |
| $(145, 49+110i)$ | $5-18i$ | $-6+5i$ |
| $(4, 1+4i)$ | $8+12i$ | $6+1i$ |
| $(1, 1)$ | $-13+6i$ | $-6i$ |
| $(96, 31+72i)$ | | |

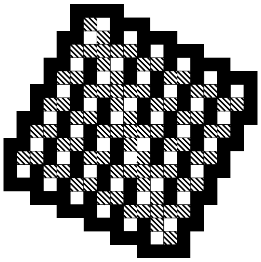
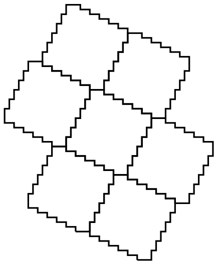

| | | |
|---|---|---|
| $(216, 17+168i)$ | | |
| $(76, 7+60i)$ | $16+6i$ | $3+6i$ |
| $(9, 1+6i)$ | $-12+9i$ | $3-5i$ |
| $(25, 1+20i)$ | $-4-15i$ | $-6-1i$ |
| $(4, 1+4i)$ | | |

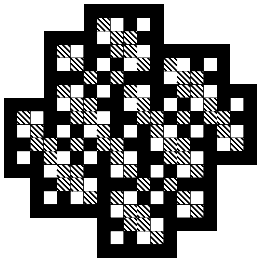
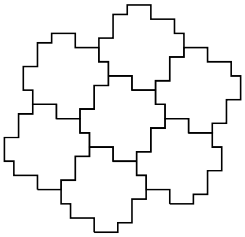

| | | |
|---|---|---|
| $(217, 49+148i)$ | | |
| $(72, 17+48i)$ | $-15+8i$ | $1-6i$ |
| $(9, 1+6i)$ | $1-15i$ | $-5+2i$ |
| $(28, 7+20i)$ | $14+7i$ | $4+4i$ |
| $(1, 1)$ | | |

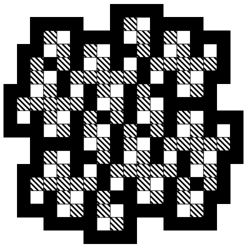
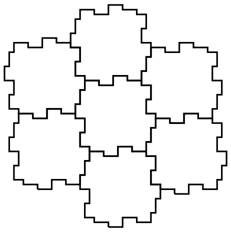

| | | |
|---|---|---|
| $(217, 49+162i)$ | | |
| $(81, 17+60i)$ | $3-17i$ | $-6+3i$ |
| $(4, 1+4i)$ | $11+10i$ | $5+3i$ |
| $(28, 7+20i)$ | $-14+7i$ | $1-6i$ |
| $(9, 1+6i)$ | | |

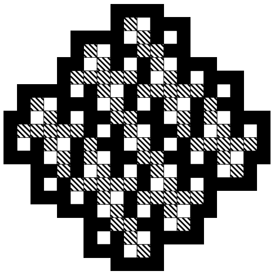
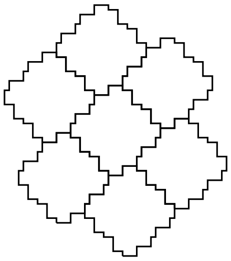

| | | |
|---|---|---|
| $(217, 97+182i)$ | | |
| $(156, 71+132i)$ | $18+7i$ | $7+6i$ |
| $(1, 1)$ | $-13+7i$ | $-7i$ |
| $(4, 1+4i)$ | $-5-14i$ | $-7+1i$ |
| $(105, 49+90i)$ | | |

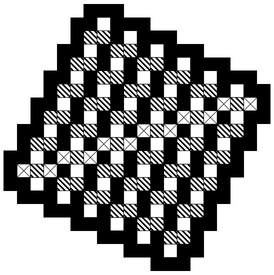
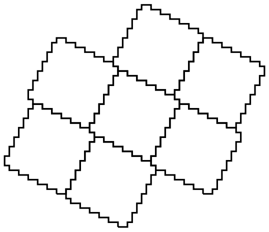

| | | |
|---|---|---|
| $(217, 145+212i)$ | | |
| $(73, 49+70i)$ | $-13+11i$ | $1-10i$ |
| $(12, 7+12i)$ | $-2-15i$ | $-8+4i$ |
| $(24, 17+24i)$ | $15+4i$ | $7+6i$ |
| $(1, 1)$ | | |

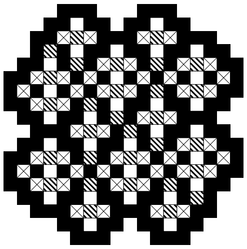
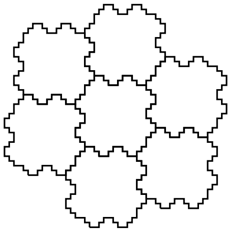

| | | |
|---|---|---|
| $(220, 49+140i)$ | | |
| $(136, 31+88i)$ | $16+10i$ | $5+4i$ |
| $(1,1)$ | $-14+5i$ | $-5i$ |
| $(9, 1+6i)$ | $-2-15i$ | $-5+1i$ |
| $(72, 17+48i)$ | | |

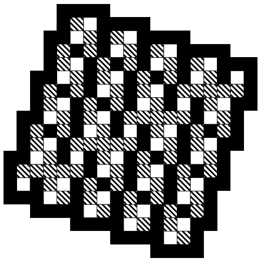

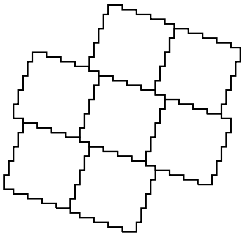

| | | |
|---|---|---|
| $(220, 199+220i)$ | | |
| $(180, 161+180i)$ | $-20i$ | $-10+9i$ |
| $(1, 1+2i)$ | $11+10i$ | $10+1i$ |
| $(1,1)$ | $-11+10i$ | $-10i$ |
| $(144, 127+144i)$ | | |

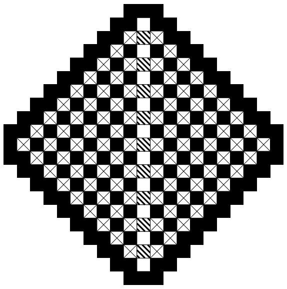

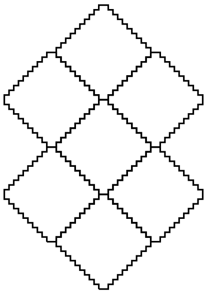

| | | |
|---|---|---|
| $(225, 1+30i)$ | | |
| $(196, 1+28i)$ | $15+14i$ | $1+1i$ |
| $(1,1)$ | $-15+1i$ | $-1i$ |
| $(0,-1)$ | $-15i$ | $-1$ |
| $(169, 1+26i)$ | | |

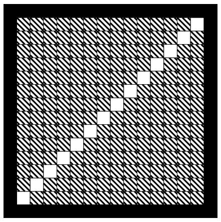

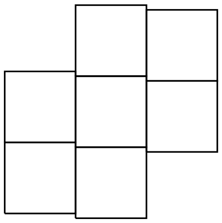

| | | |
|---|---|---|
| $(225, 1+60i)$ | | |
| $(64, 1+16i)$ | $-15+8i$ | $1-2i$ |
| $(0,-1)$ | $-15i$ | $-2$ |
| $(49, 1+14i)$ | $15+7i$ | $1+2i$ |
| $(1,1)$ | | |

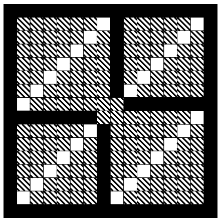

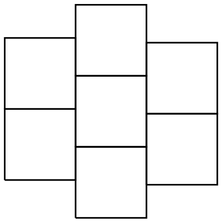

| | | |
|---|---|---|
| $(225, 1+120i)$ | | |
| $(121, 1+66i)$ | $15+11i$ | $3+4i$ |
| $(16, 1+8i)$ | $-15+4i$ | $1-4i$ |
| $(0,-1)$ | $-15i$ | $-4$ |
| $(49, 1+28i)$ | | |

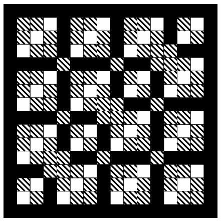

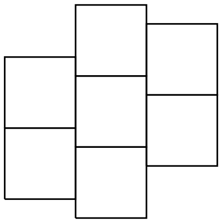

| | | |
|---|---|---|
| $(225, 1+210i)$ | | |
| $(169, 1+156i)$ | $-15+13i$ | $6-7i$ |
| $(0,-1)$ | $-15i$ | $-7$ |
| $(4, 1+4i)$ | $15+2i$ | $1+7i$ |
| $(121, 1+110i)$ | | |

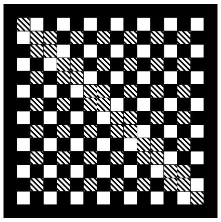

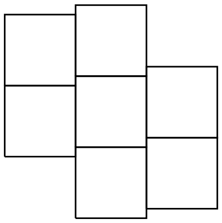

| | | |
|---|---|---|
| $(228, 7+60i)$ | | |
| $(64, 1+16i)$ | $6-16i$ | $-2+1i$ |
| $(49, 1+14i)$ | $9+14i$ | $2+1i$ |
| $(1,1)$ | $-15+2i$ | $-2i$ |
| $(0,-1)$ | | |

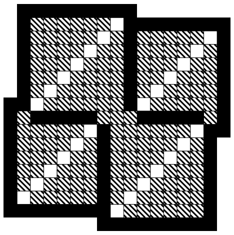

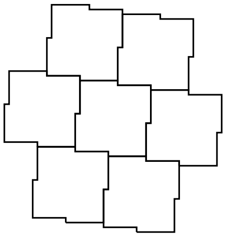

| | | |
|---|---|---|
| $(232, 49+168i)$ | | |
| $(81, 17+60i)$ | $12+13i$ | $6+3i$ |
| $(28, 7+20i)$ | $-16+2i$ | $-1-6i$ |
| $(9, 1+6i)$ | $4-15i$ | $-5+3i$ |
| $(4, 1+4i)$ | | |

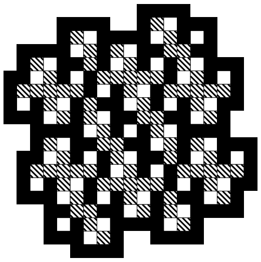
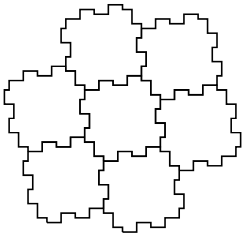

| | | |
|---|---|---|
| $(232, 127+208i)$ | | |
| $(88, 49+80i)$ | $16+8i$ | $8+5i$ |
| $(1, 1)$ | $-13+8i$ | $-8i$ |
| $(33, 17+30i)$ | $-3-16i$ | $-8+3i$ |
| $(12, 7+12i)$ | | |

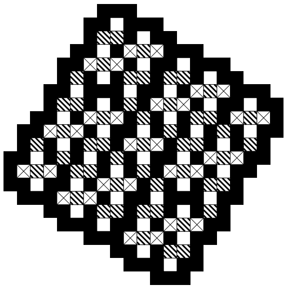
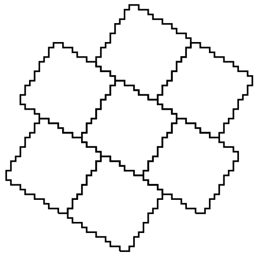

| | | |
|---|---|---|
| $(240, 31+120i)$ | | |
| $(129, 17+66i)$ | $15+12i$ | $4+3i$ |
| $(1, 1)$ | $-15+4i$ | $-4i$ |
| $(16, 1+8i)$ | $-16i$ | $-4+1i$ |
| $(52, 7+28i)$ | | |

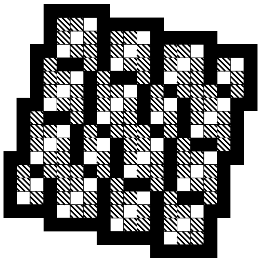
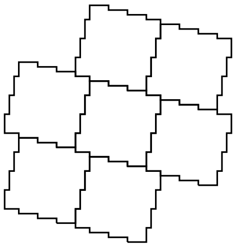

| | | |
|---|---|---|
| $(244, 7+108i)$ | | |
| $(81, 1+36i)$ | $-1-18i$ | $-4$ |
| $(16, 1+8i)$ | $14+8i$ | $2+3i$ |
| $(25, 1+10i)$ | $-13+10i$ | $2-3i$ |
| $(0, -1)$ | | |

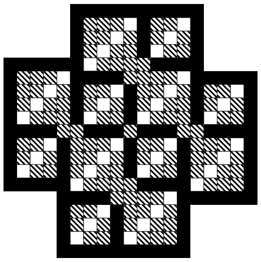
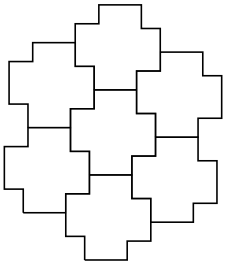

| | | |
|---|---|---|
| $(249, 17+108i)$ | | |
| $(84, 7+36i)$ | $-18+3i$ | $-4i$ |
| $(25, 1+10i)$ | $7-15i$ | $-3+2i$ |
| $(16, 1+8i)$ | $11+12i$ | $3+2i$ |
| $(1, 1)$ | | |

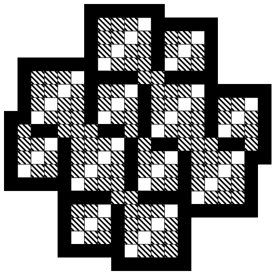
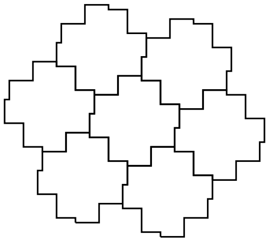

| | | |
|---|---|---|
| $(249, 161+234i)$ | | |
| $(148, 97+140i)$ | $19+6i$ | $9+7i$ |
| $(1, 1)$ | $-13+9i$ | $-9i$ |
| $(12, 7+12i)$ | $-6-15i$ | $-9+2i$ |
| $(73, 49+70i)$ | | |

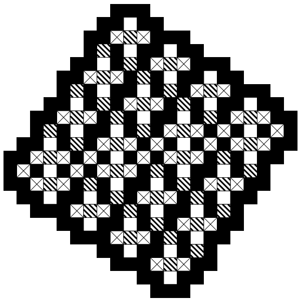
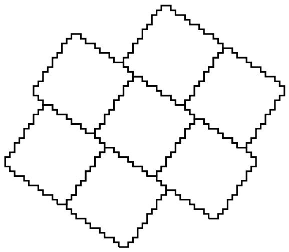

| | | |
|---|---|---|
| $(256, 1+32i)$ | | |
| $(225, 1+30i)$ | $16+15i$ | $1+1i$ |
| $(1, 1)$ | $-16+1i$ | $-1i$ |
| $(0, -1)$ | $-16i$ | $-1$ |
| $(196, 1+28i)$ | | |

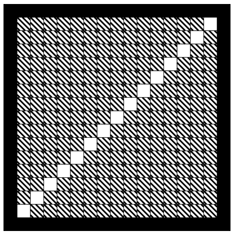
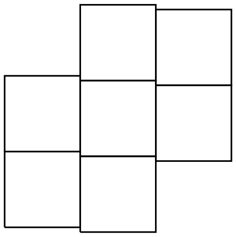

| | | |
|---|---|---|
| $(256, 1+96i)$ | | |
| $(121, 1+44i)$ | $-16+11i$ | $2-3i$ |
| $(0, -1)$ | $-16i$ | $-3$ |
| $(25, 1+10i)$ | $16+5i$ | $1+3i$ |
| $(36, 1+12i)$ | | |

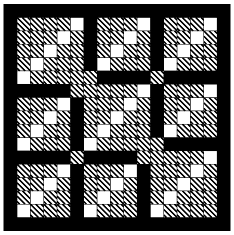
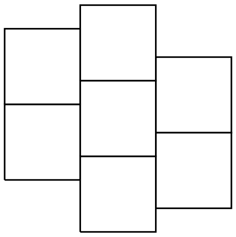

| | | |
|---|---|---|
| $(256, 1+160i)$ | | |
| $(169, 1+104i)$ | $-16+13i$ | $4-5i$ |
| $(0, -1)$ | $-16i$ | $-5$ |
| $(9, 1+6i)$ | $16+3i$ | $1+5i$ |
| $(100, 1+60i)$ | | |

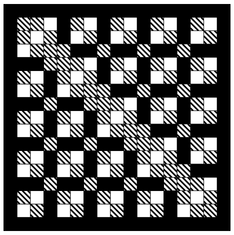
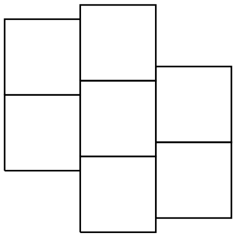

| | | |
|---|---|---|
| $(256, 31+200i)$ | | |
| $(153, 17+120i)$ | $-3-20i$ | $-8$ |
| $(4, 1+4i)$ | $14+8i$ | $4+5i$ |
| $(9, 1+6i)$ | $-11+12i$ | $4-5i$ |
| $(76, 7+60i)$ | | |

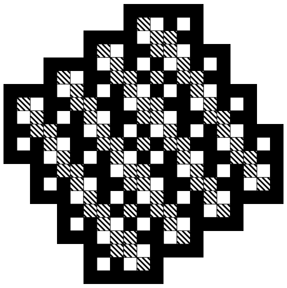
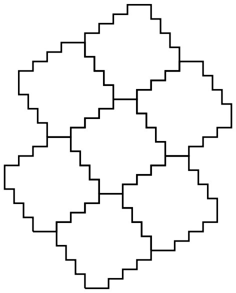

| | | |
|---|---|---|
| $(256, 1+224i)$ | | |
| $(81, 1+72i)$ | $16+9i$ | $4+7i$ |
| $(49, 1+42i)$ | $-16+7i$ | $3-7i$ |
| $(0, -1)$ | $-16i$ | $-7$ |
| $(4, 1+4i)$ | | |

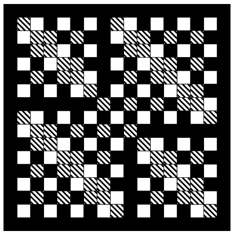
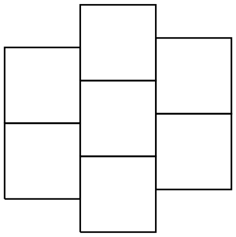

| | | |
|---|---|---|
| $(256, 127+240i)$ | | |
| $(97, 49+92i)$ | $17+8i$ | $8+6i$ |
| $(33, 17+30i)$ | $-15+8i$ | $-9i$ |
| $(4, 1+4i)$ | $-2-16i$ | $-8+3i$ |
| $(12, 7+12i)$ | | |

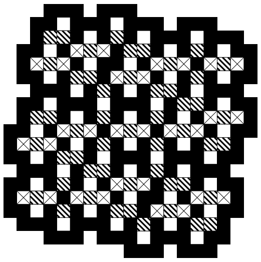
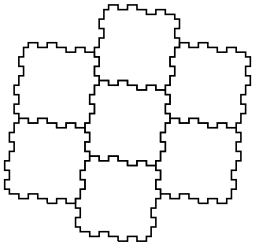

| | | |
|---|---|---|
| $(264, 17+96i)$ | | |
| $(124, 7+44i)$ | $8-18i$ | $-3+2i$ |
| $(25, 1+10i)$ | $8+15i$ | $3+1i$ |
| $(1,1)$ | $-16+3i$ | $-3i$ |
| $(36, 1+12i)$ | | |

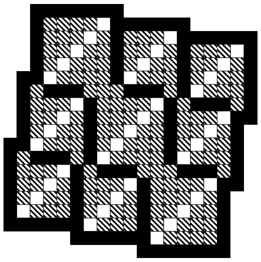
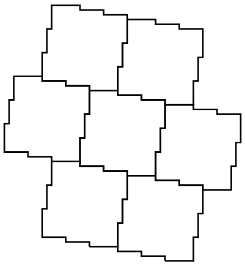

| | | |
|---|---|---|
| $(264, 241+264i)$ | | |
| $(220, 199+220i)$ | $-22i$ | $-11+10i$ |
| $(1, 1+2i)$ | $12+11i$ | $11+1i$ |
| $(1,1)$ | $-12+11i$ | $-11i$ |
| $(180, 161+180i)$ | | |

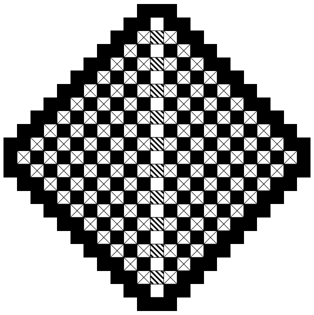
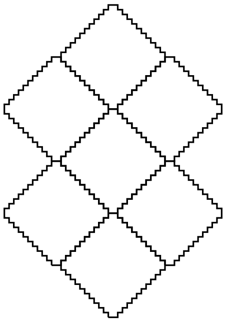

| | | |
|---|---|---|
| $(265, 49+200i)$ | | |
| $(160, 31+120i)$ | $-20+5i$ | $-8i$ |
| $(9, 1+6i)$ | $7-15i$ | $-5+4i$ |
| $(4, 1+4i)$ | $13+10i$ | $5+4i$ |
| $(81, 17+60i)$ | | |

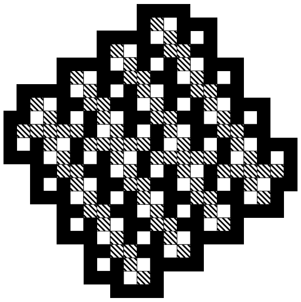
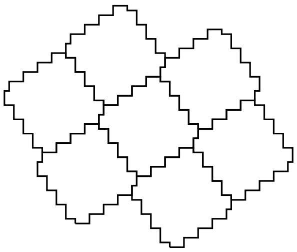

| | | |
|---|---|---|
| $(265, 145+244i)$ | | |
| $(88, 49+80i)$ | $-17+8i$ | $-1-10i$ |
| $(33, 17+30i)$ | $3-17i$ | $-7+6i$ |
| $(12, 7+12i)$ | $14+9i$ | $8+4i$ |
| $(1,1)$ | | |

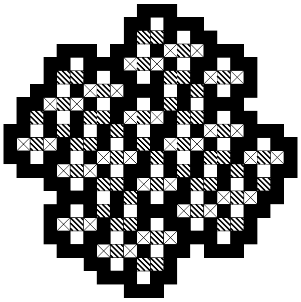
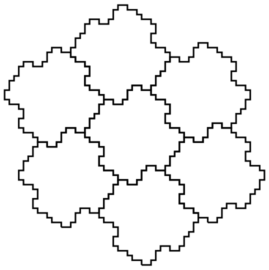

| | | |
|---|---|---|
| $(268, 7+236i)$ | | |
| $(81, 1+72i)$ | $-5-18i$ | $-8-2i$ |
| $(4, 1+4i)$ | $16+4i$ | $2+7i$ |
| $(49, 1+42i)$ | $-11+14i$ | $6-5i$ |
| $(0,-1)$ | | |

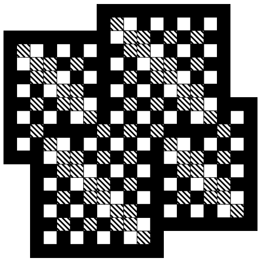
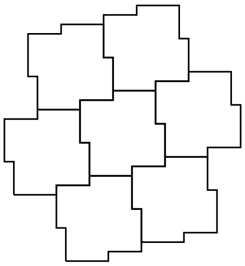

| | | |
|---|---|---|
| $(268, 199+260i)$ | | |
| $(129, 97+126i)$ | $19+6i$ | $10+7i$ |
| $(1,1)$ | $-13+10i$ | $-10i$ |
| $(24, 17+24i)$ | $-6-16i$ | $-10+3i$ |
| $(40, 31+40i)$ | | |

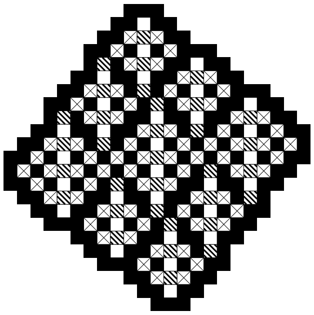
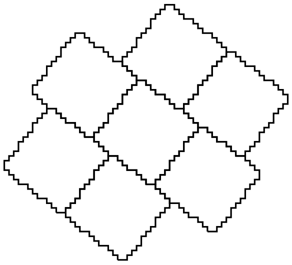

| | | |
|---|---|---|
| $(273, 97+210i)$ | | |
| $(204, 71+156i)$ | $6-21i$ | $-7+6i$ |
| $(4, 1+4i)$ | $9+14i$ | $7+1i$ |
| $(1,1)$ | $-15+7i$ | $-7i$ |
| $(145, 49+110i)$ | | |

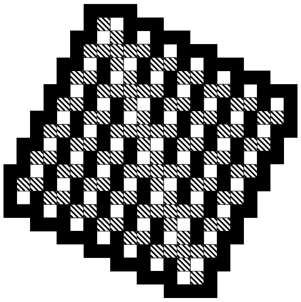
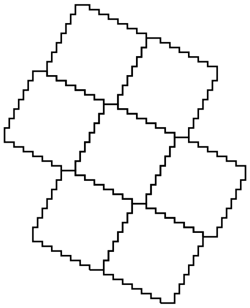

| | | |
|---|---|---|
| $(276, 161+252i)$ | | |
| $(169, 97+154i)$ | $2-21i$ | $-9+7i$ |
| $(12, 7+12i)$ | $12+12i$ | $9+2i$ |
| $(1,1)$ | $-14+9i$ | $-9i$ |
| $(88, 49+80i)$ | | |

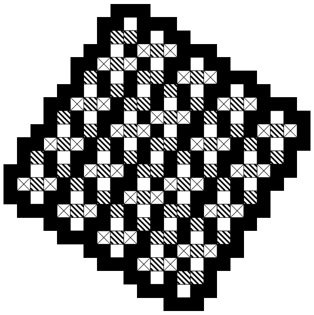
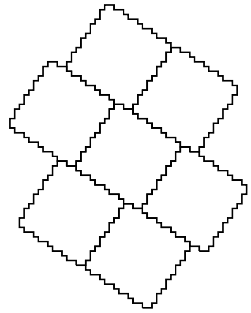

| | | |
|---|---|---|
| $(280, 49+160i)$ | | |
| $(184, 31+104i)$ | $8-20i$ | $-5+4i$ |
| $(9, 1+6i)$ | $8+15i$ | $5+1i$ |
| $(1,1)$ | $-16+5i$ | $-5i$ |
| $(108, 17+60i)$ | | |

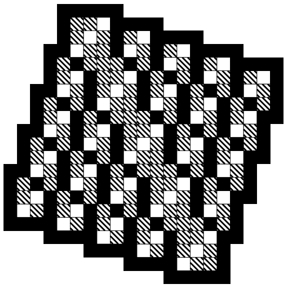
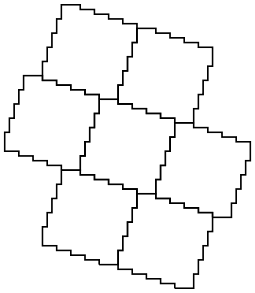

| | | |
|---|---|---|
| $(280, 145+264i)$ | | |
| $(97, 49+92i)$ | $-4-19i$ | $-10+3i$ |
| $(12, 7+12i)$ | $16+6i$ | $7+6i$ |
| $(33, 17+30i)$ | $-12+13i$ | $3-9i$ |
| $(4, 1+4i)$ | | |

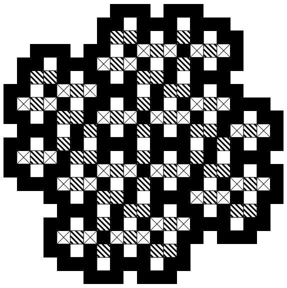
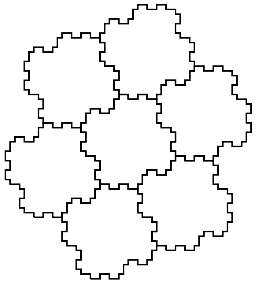

| | | |
|---|---|---|
| $(288, 127+240i)$ | | |
| $(217, 97+182i)$ | $21+8i$ | $8+7i$ |
| $(1,1)$ | $-15+8i$ | $-8i$ |
| $(4, 1+4i)$ | $-6-16i$ | $-8+1i$ |
| $(156, 71+132i)$ | | |

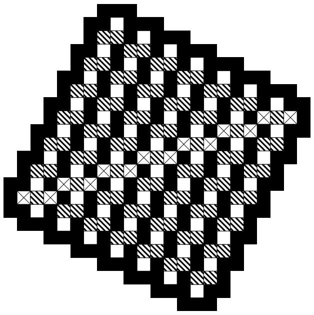
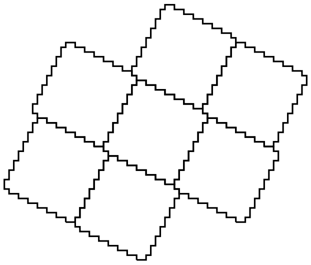

| | | |
|---|---|---|
| $(289, 1+34i)$ | | |
| $(256, 1+32i)$ | $17+16i$ | $1+1i$ |
| $(1,1)$ | $-17+1i$ | $-1i$ |
| $(0,-1)$ | $-17i$ | $-1$ |
| $(225, 1+30i)$ | | |

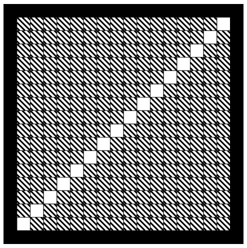
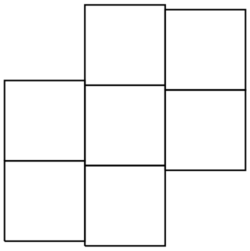

| | | |
|---|---|---|
| $(289, 1+68i)$ | | |
| $(81, 1+18i)$ | $-17+9i$ | $1-2i$ |
| $(0,-1)$ | $-17i$ | $-2$ |
| $(64, 1+16i)$ | $17+8i$ | $1+2i$ |
| $(1,1)$ | | |

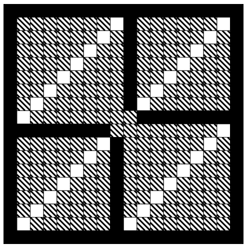
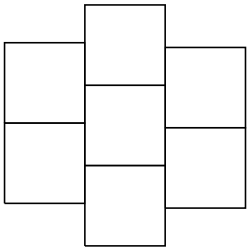

| | | |
|---|---|---|
| $(289, 1+102i)$ | | |
| $(121, 1+44i)$ | $17+11i$ | $2+3i$ |
| $(36, 1+12i)$ | $-17+6i$ | $1-3i$ |
| $(0,-1)$ | $-17i$ | $-3$ |
| $(25, 1+10i)$ | | |

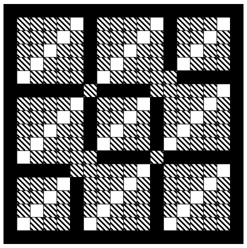
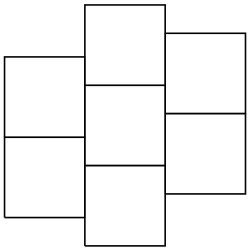

| | | |
|---|---|---|
| $(289, 1+136i)$ | | |
| $(169, 1+78i)$ | $-17+13i$ | $3-4i$ |
| $(0,-1)$ | $-17i$ | $-4$ |
| $(16, 1+8i)$ | $17+4i$ | $1+4i$ |
| $(81, 1+36i)$ | | |

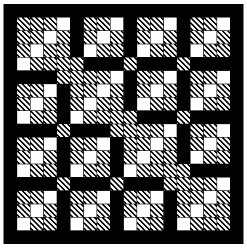
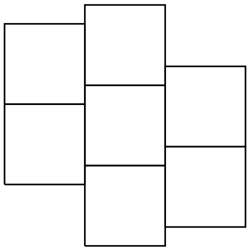

| | | |
|---|---|---|
| $(289, 1+170i)$ | | |
| $(100, 1+60i)$ | $17+10i$ | $3+5i$ |
| $(49, 1+28i)$ | $-17+7i$ | $2-5i$ |
| $(0,-1)$ | $-17i$ | $-5$ |
| $(9, 1+6i)$ | | |

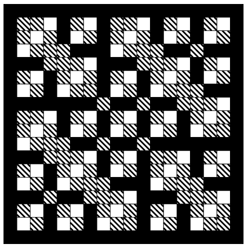
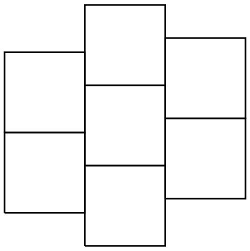

| | | |
|---|---|---|
| $(289, 1+204i)$ | | |
| $(196, 1+140i)$ | $17+14i$ | $5+6i$ |
| $(9, 1+6i)$ | $-17+3i$ | $1-6i$ |
| $(0, -1)$ | $-17i$ | $-6$ |
| $(121, 1+88i)$ | | |

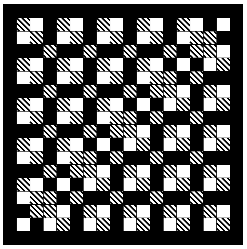
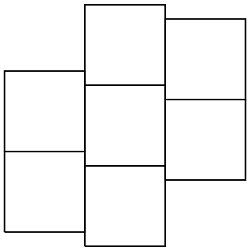

| | | |
|---|---|---|
| $(289, 1+238i)$ | | |
| $(144, 1+120i)$ | $17+12i$ | $5+7i$ |
| $(25, 1+20i)$ | $-17+5i$ | $2-7i$ |
| $(0, -1)$ | $-17i$ | $-7$ |
| $(49, 1+42i)$ | | |

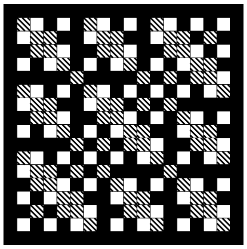
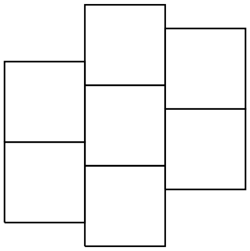

| | | |
|---|---|---|
| $(289, 1+272i)$ | | |
| $(225, 1+210i)$ | $-17+15i$ | $7-8i$ |
| $(0, -1)$ | $-17i$ | $-8$ |
| $(4, 1+4i)$ | $17+2i$ | $1+8i$ |
| $(169, 1+156i)$ | | |

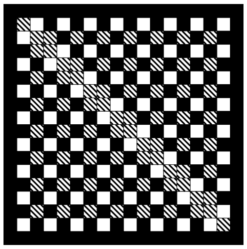
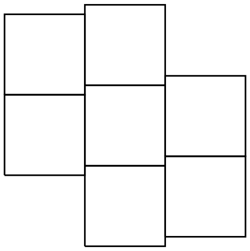

| | | |
|---|---|---|
| $(289, 241+286i)$ | | |
| $(84, 71+84i)$ | $18+7i$ | $11+6i$ |
| $(1, 1)$ | $-13+11i$ | $-11i$ |
| $(60, 49+60i)$ | $-5-18i$ | $-11+5i$ |
| $(1, 1+2i)$ | | |

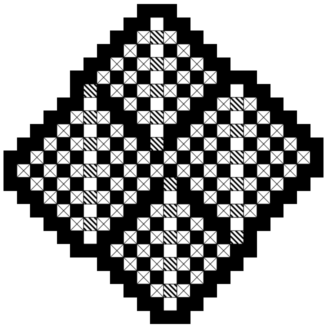
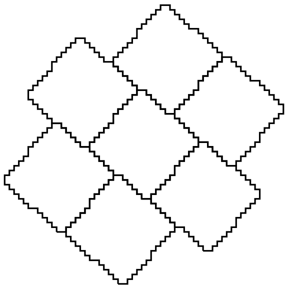

| | | |
|---|---|---|
| $(292, 7+68i)$ | | |
| $(81, 1+18i)$ | $7-18i$ | $-2+1i$ |
| $(64, 1+16i)$ | $10+16i$ | $2+1i$ |
| $(1, 1)$ | $-17+2i$ | $-2i$ |
| $(0, -1)$ | | |

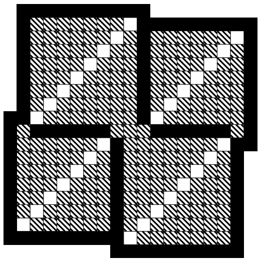
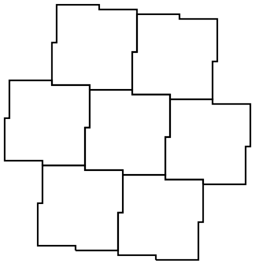

| | | |
|---|---|---|
| $(297, 17+102i)$ | | |
| $(124, 7+44i)$ | $14+15i$ | $3+2i$ |
| $(1, 1)$ | $-17+3i$ | $-3i$ |
| $(36, 1+12i)$ | $3-18i$ | $-3+1i$ |
| $(25, 1+10i)$ | | |

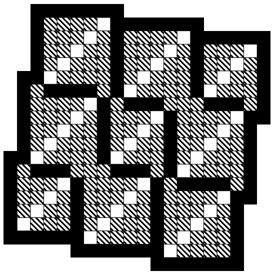
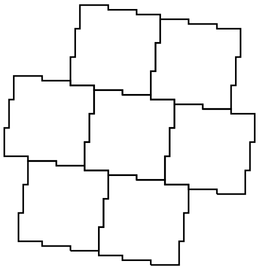

| | | |
|---|---|---|
| $(297, 17+168i)$ | | |
| $(148, 7+84i)$ | $-2-21i$ | $-6$ |
| $(9, 1+6i)$ | $15+9i$ | $3+4i$ |
| $(16, 1+8i)$ | $-13+12i$ | $3-4i$ |
| $(49, 1+28i)$ | | |

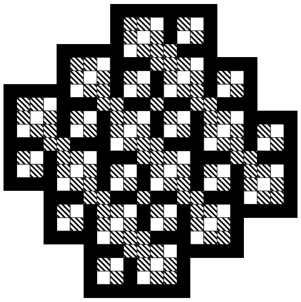
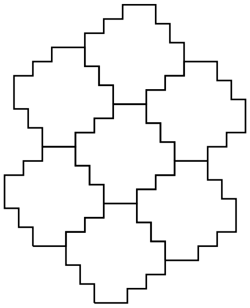

| | | |
|---|---|---|
| $(304, 31+136i)$ | | |
| $(177, 17+78i)$ | $9-20i$ | $-4+3i$ |
| $(16, 1+8i)$ | $8+16i$ | $4+1i$ |
| $(1, 1)$ | $-17+4i$ | $-4i$ |
| $(84, 7+36i)$ | | |

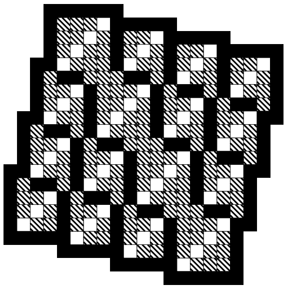
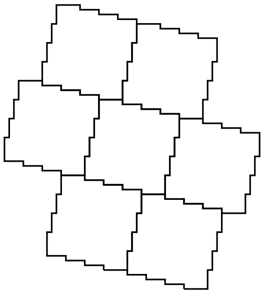

| | | |
|---|---|---|
| $(304, 31+168i)$ | | |
| $(153, 17+84i)$ | $-21+4i$ | $-6i$ |
| $(16, 1+8i)$ | $8-16i$ | $-4+3i$ |
| $(9, 1+6i)$ | $13+12i$ | $4+3i$ |
| $(52, 7+28i)$ | | |

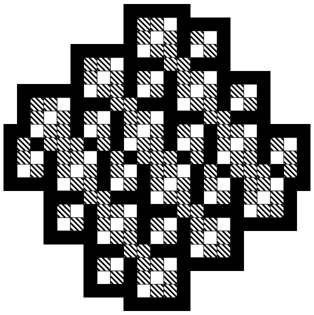
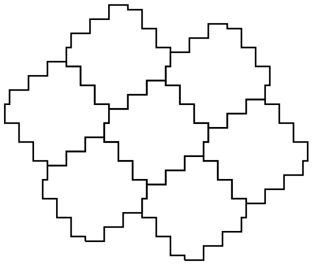

| | | |
|---|---|---|
| $(304, 97+224i)$ | | |
| $(96, 31+72i)$ | $16+12i$ | $7+4i$ |
| $(1, 1)$ | $-16+7i$ | $-7i$ |
| $(57, 17+42i)$ | $-19i$ | $-7+3i$ |
| $(4, 1+4i)$ | | |

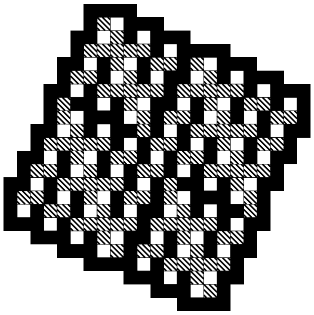
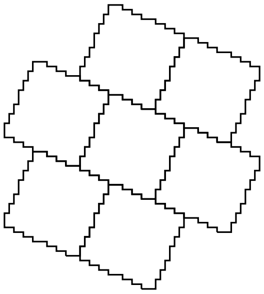

| | | |
|---|---|---|
| $(312, 287+312i)$ | | |
| $(264, 241+264i)$ | $-24i$ | $-12+11i$ |
| $(1, 1+2i)$ | $13+12i$ | $12+1i$ |
| $(1, 1)$ | $-13+12i$ | $-12i$ |
| $(220, 199+220i)$ | | |

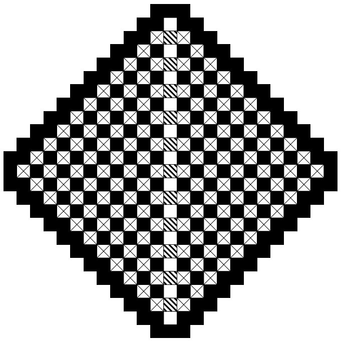
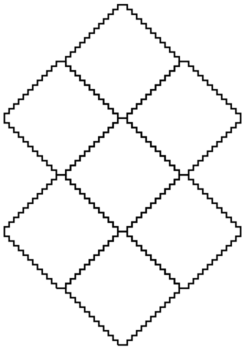

| | | |
|---|---|---|
| $(313, 49+170i)$ | | |
| $(108, 17+60i)$ | $15+14i$ | $5+3i$ |
| $(1,1)$ | $-17+5i$ | $-5i$ |
| $(52, 7+28i)$ | $2-19i$ | $-5+2i$ |
| $(9, 1+6i)$ | | |

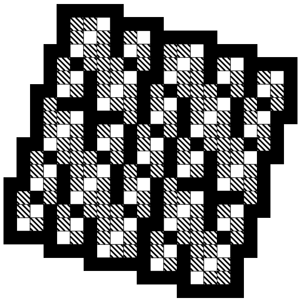
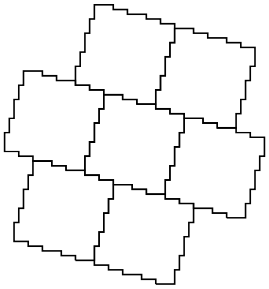

| | | |
|---|---|---|
| $(313, 97+236i)$ | | |
| $(96, 31+72i)$ | $-20+3i$ | $-2-8i$ |
| $(57, 17+42i)$ | $9-17i$ | $-5+6i$ |
| $(4, 1+4i)$ | $11+14i$ | $7+2i$ |
| $(1,1)$ | | |

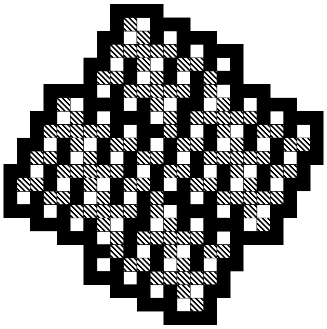
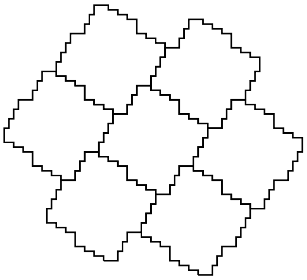

| | | |
|---|---|---|
| $(316, 7+188i)$ | | |
| $(100, 1+60i)$ | $-4-20i$ | $-6-1i$ |
| $(9, 1+6i)$ | $17+6i$ | $2+5i$ |
| $(49, 1+28i)$ | $-13+14i$ | $4-4i$ |
| $(0,-1)$ | | |

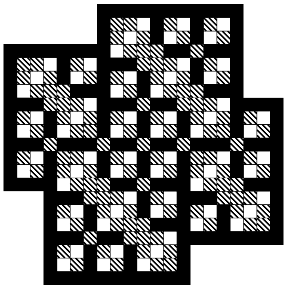
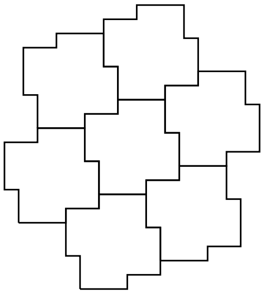

| | | |
|---|---|---|
| $(316, 241+308i)$ | | |
| $(129, 97+126i)$ | $-2-21i$ | $-11+7i$ |
| $(40, 31+40i)$ | $16+10i$ | $11+4i$ |
| $(1,1)$ | $-14+11i$ | $-11i$ |
| $(24, 17+24i)$ | | |

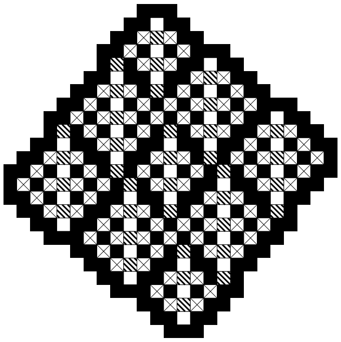
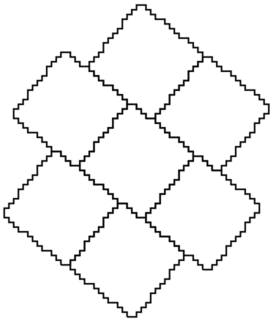

| | | |
|---|---|---|
| $(321, 17+270i)$ | | |
| $(156, 7+132i)$ | $-6-21i$ | $-9-2i$ |
| $(4, 1+4i)$ | $17+6i$ | $3+7i$ |
| $(25, 1+20i)$ | $-11+15i$ | $6-5i$ |
| $(49, 1+42i)$ | | |

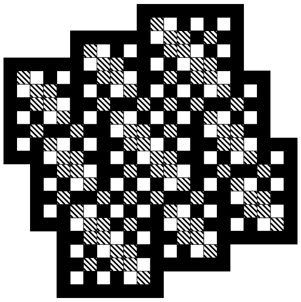
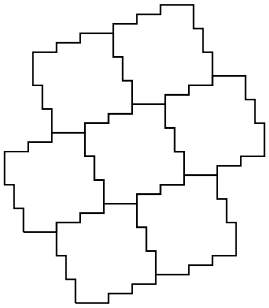

| | | |
|---|---|---|
| $(321, 161+312i)$ | | |
| $(193, 97+186i)$ | $-17+15i$ | $3-12i$ |
| $(4, 1+4i)$ | $-1-18i$ | $-9+4i$ |
| $(12, 7+12i)$ | $18+3i$ | $6+8i$ |
| $(97, 49+92i)$ | | |

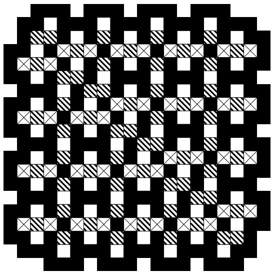

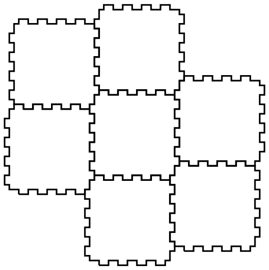

| | | |
|---|---|---|
| $(324, 1+36i)$ | | |
| $(289, 1+34i)$ | $18+17i$ | $1+1i$ |
| $(1, 1)$ | $-18+1i$ | $-1i$ |
| $(0, -1)$ | $-18i$ | $-1$ |
| $(256, 1+32i)$ | | |

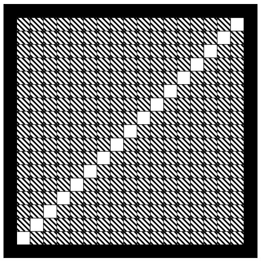

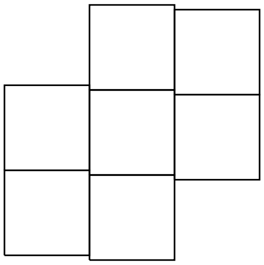

| | | |
|---|---|---|
| $(324, 1+180i)$ | | |
| $(121, 1+66i)$ | $-18+11i$ | $3-5i$ |
| $(0, -1)$ | $-18i$ | $-5$ |
| $(49, 1+28i)$ | $18+7i$ | $2+5i$ |
| $(16, 1+8i)$ | | |

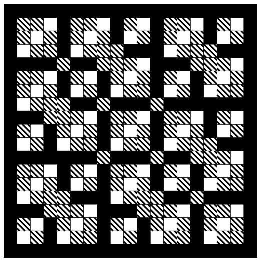

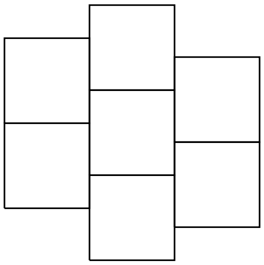

| | | |
|---|---|---|
| $(324, 71+204i)$ | | |
| $(220, 49+140i)$ | $20+12i$ | $6+5i$ |
| $(1, 1)$ | $-17+6i$ | $-6i$ |
| $(9, 1+6i)$ | $-3-18i$ | $-6+1i$ |
| $(136, 31+88i)$ | | |

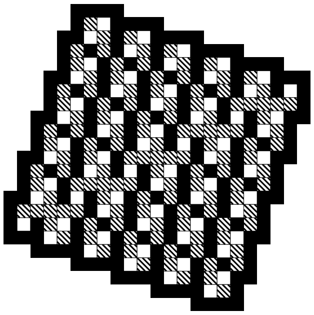

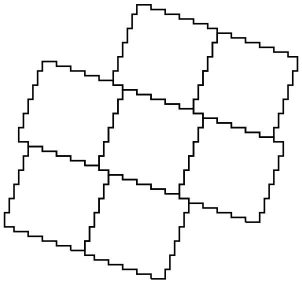

| | | |
|---|---|---|
| $(324, 1+252i)$ | | |
| $(169, 1+130i)$ | $-18+13i$ | $5-7i$ |
| $(0, -1)$ | $-18i$ | $-7$ |
| $(25, 1+20i)$ | $18+5i$ | $2+7i$ |
| $(64, 1+48i)$ | | |

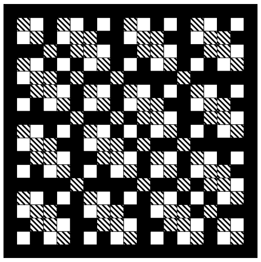

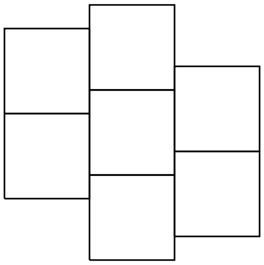

| | | |
|---|---|---|
| $(336, 161+288i)$ | | |
| $(105, 49+90i)$ | $-21i$ | $-9+5i$ |
| $(64, 31+56i)$ | $16+12i$ | $9+4i$ |
| $(1, 1)$ | $-16+9i$ | $-9i$ |
| $(4, 1+4i)$ | | |

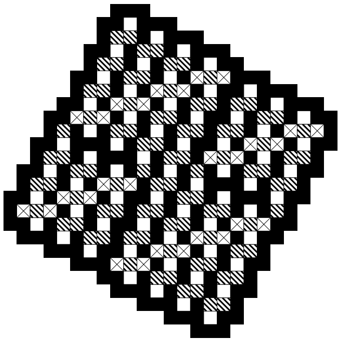

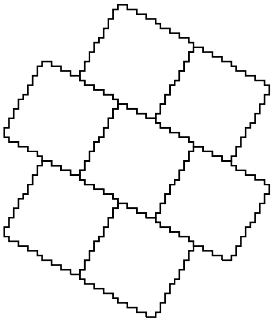

| | | |
|---|---|---|
| $(337, 49+188i)$ | | |
| $(108, 17+60i)$ | $-21+2i$ | $-1-6i$ |
| $(52, 7+28i)$ | $10-17i$ | $-4+4i$ |
| $(9, 1+6i)$ | $11+15i$ | $5+2i$ |
| $(1, 1)$ | | |

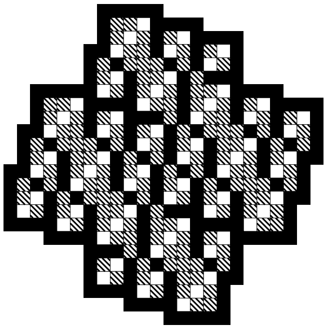

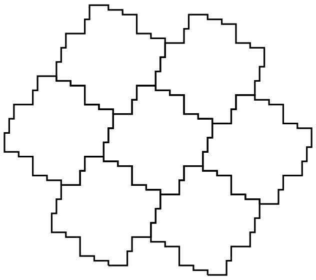

| | | |
|---|---|---|
| $(337, 97+238i)$ | | |
| $(168, 49+120i)$ | $19+12i$ | $7+5i$ |
| $(1, 1)$ | $-17+7i$ | $-7i$ |
| $(28, 7+20i)$ | $-2-19i$ | $-7+2i$ |
| $(57, 17+42i)$ | | |

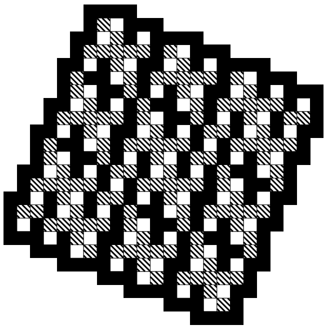

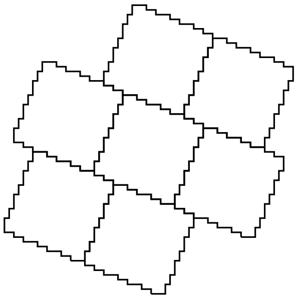

| | | |
|---|---|---|
| $(345, 161+300i)$ | | |
| $(105, 49+90i)$ | $-15+15i$ | $3-10i$ |
| $(4, 1+4i)$ | $-5-18i$ | $-9+2i$ |
| $(64, 31+56i)$ | $20+3i$ | $6+8i$ |
| $(1, 1)$ | | |

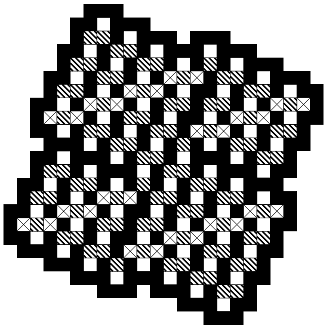

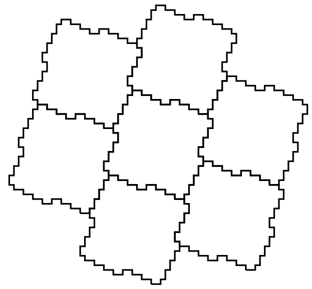

| | | |
|---|---|---|
| $(345, 241+330i)$ | | |
| $(184, 127+176i)$ | $-23i$ | $-11+8i$ |
| $(24, 17+24i)$ | $15+12i$ | $11+3i$ |
| $(1, 1)$ | $-15+11i$ | $-11i$ |
| $(73, 49+70i)$ | | |

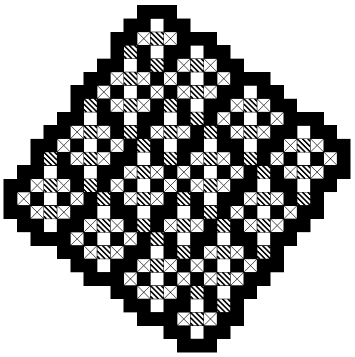

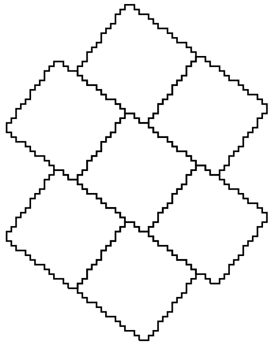

| | | |
|---|---|---|
| $(348, 49+180i)$ | | |
| $(129, 17+66i)$ | $6-21i$ | $-5+3i$ |
| $(52, 7+28i)$ | $12+16i$ | $5+2i$ |
| $(1, 1)$ | $-18+5i$ | $-5i$ |
| $(16, 1+8i)$ | | |

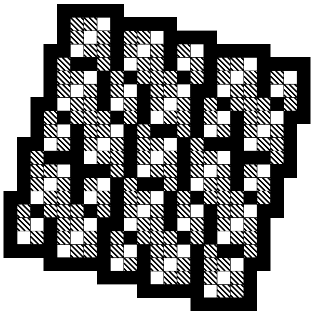

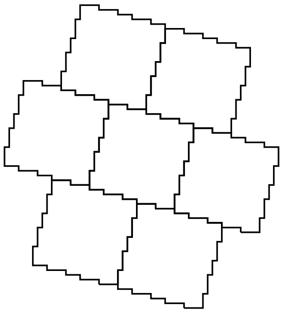

| | | |
|---|---|---|
| $(352, 127+272i)$ | | |
| $(273, 97+210i)$ | $7-24i$ | $-8+7i$ |
| $(4, 1+4i)$ | $10+16i$ | $8+1i$ |
| $(1, 1)$ | $-17+8i$ | $-8i$ |
| $(204, 71+156i)$ | | |

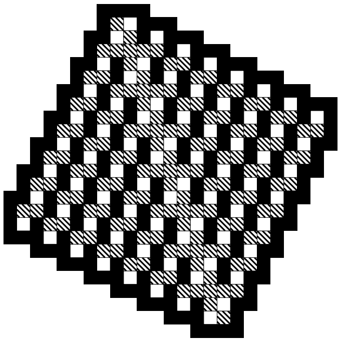

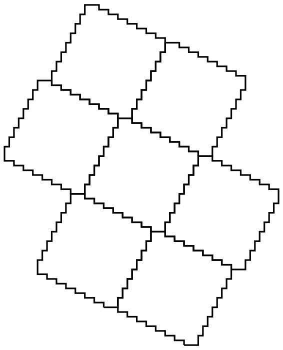

| | | |
|---|---|---|
| $(361, 1+38i)$ | | |
| $(324, 1+36i)$ | $19+18i$ | $1+1i$ |
| $(1, 1)$ | $-19+1i$ | $-1i$ |
| $(0, -1)$ | $-19i$ | $-1$ |
| $(289, 1+34i)$ | | |

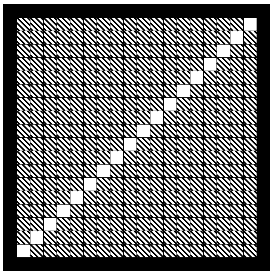

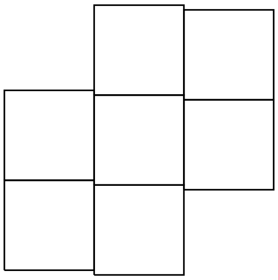

| | | |
|---|---|---|
| $(361, 1+76i)$ | | |
| $(100, 1+20i)$ | $-19+10i$ | $1-2i$ |
| $(0, -1)$ | $-19i$ | $-2$ |
| $(81, 1+18i)$ | $19+9i$ | $1+2i$ |
| $(1, 1)$ | | |

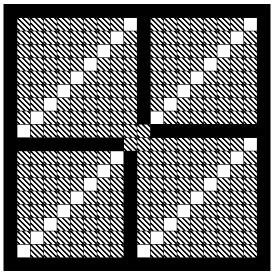

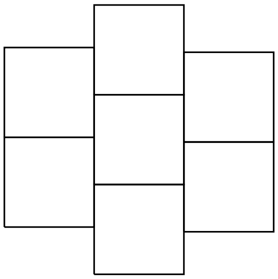

| | | |
|---|---|---|
| $(361, 1+114i)$ | | |
| $(169, 1+52i)$ | $-19+13i$ | $2-3i$ |
| $(0, -1)$ | $-19i$ | $-3$ |
| $(36, 1+12i)$ | $19+6i$ | $1+3i$ |
| $(49, 1+14i)$ | | |

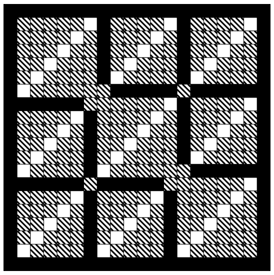

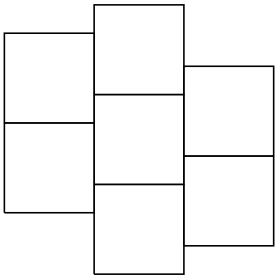

| | | |
|---|---|---|
| $(361, 1+152i)$ | | |
| $(196, 1+84i)$ | $19+14i$ | $3+4i$ |
| $(25, 1+10i)$ | $-19+5i$ | $1-4i$ |
| $(0, -1)$ | $-19i$ | $-4$ |
| $(81, 1+36i)$ | | |

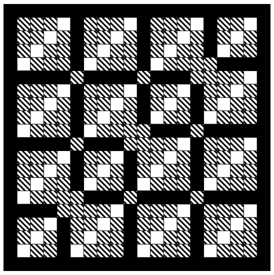
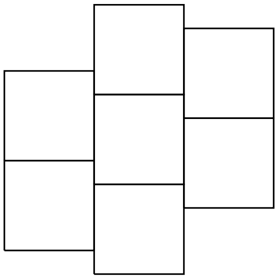

| | | |
|---|---|---|
| $(361, 1+190i)$ | | |
| $(225, 1+120i)$ | $19+15i$ | $4+5i$ |
| $(16, 1+8i)$ | $-19+4i$ | $1-5i$ |
| $(0, -1)$ | $-19i$ | $-5$ |
| $(121, 1+66i)$ | | |

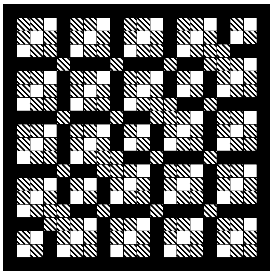
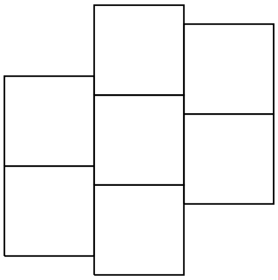

| | | |
|---|---|---|
| $(361, 1+228i)$ | | |
| $(256, 1+160i)$ | $-19+16i$ | $5-6i$ |
| $(0, -1)$ | $-19i$ | $-6$ |
| $(9, 1+6i)$ | $19+3i$ | $1+6i$ |
| $(169, 1+104i)$ | | |

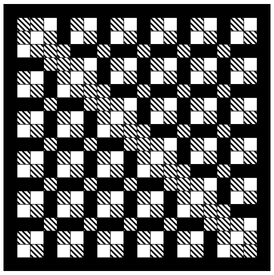
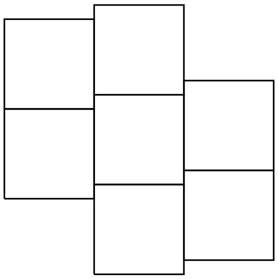

| | | |
|---|---|---|
| $(361, 1+266i)$ | | |
| $(121, 1+88i)$ | $-19+11i$ | $4-7i$ |
| $(0, -1)$ | $-19i$ | $-7$ |
| $(64, 1+48i)$ | $19+8i$ | $3+7i$ |
| $(9, 1+6i)$ | | |

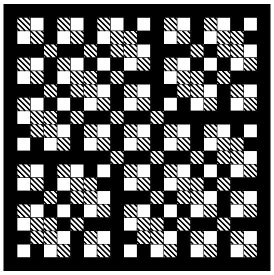
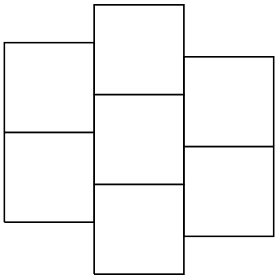

| | | |
|---|---|---|
| $(361, 97+270i)$ | | |
| $(177, 49+132i)$ | $-23+3i$ | $-2-9i$ |
| $(28, 7+20i)$ | $10-17i$ | $-5+6i$ |
| $(4, 1+4i)$ | $13+14i$ | $7+3i$ |
| $(57, 17+42i)$ | | |

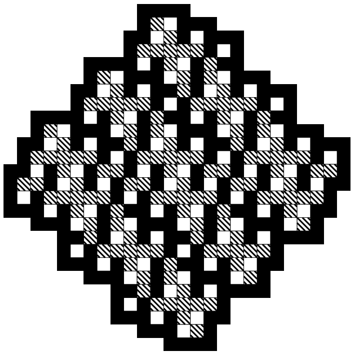
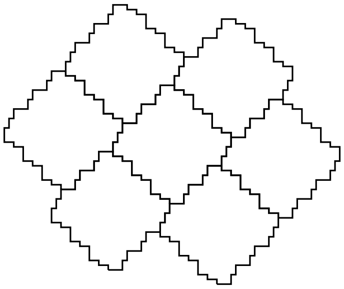

| | | |
|---|---|---|
| $(361, 1+304i)$ | | |
| $(144, 1+120i)$ | $-19+12i$ | $5-8i$ |
| $(0, -1)$ | $-19i$ | $-8$ |
| $(49, 1+42i)$ | $19+7i$ | $3+8i$ |
| $(25, 1+20i)$ | | |

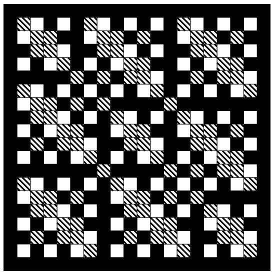

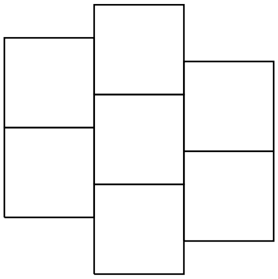

| | | |
|---|---|---|
| $(361, 1+342i)$ | | |
| $(289, 1+272i)$ | $-19+17i$ | $8-9i$ |
| $(0, -1)$ | $-19i$ | $-9$ |
| $(4, 1+4i)$ | $19+2i$ | $1+9i$ |
| $(225, 1+210i)$ | | |

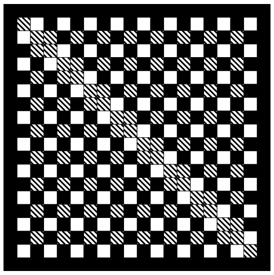

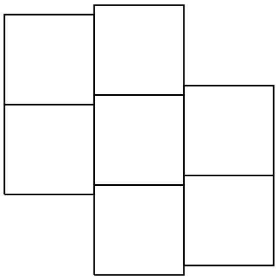

| | | |
|---|---|---|
| $(364, 7+76i)$ | | |
| $(100, 1+20i)$ | $8-20i$ | $-2+1i$ |
| $(81, 1+18i)$ | $11+18i$ | $2+1i$ |
| $(1, 1)$ | $-19+2i$ | $-2i$ |
| $(0, -1)$ | | |

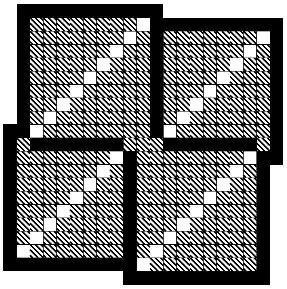

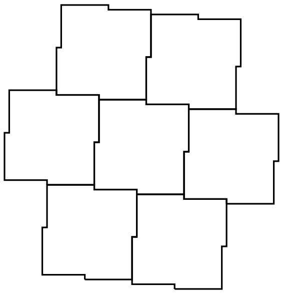

| | | |
|---|---|---|
| $(364, 7+132i)$ | | |
| $(121, 1+44i)$ | $-1-22i$ | $-4$ |
| $(25, 1+10i)$ | $17+10i$ | $2+3i$ |
| $(36, 1+12i)$ | $-16+12i$ | $2-3i$ |
| $(0, -1)$ | | |

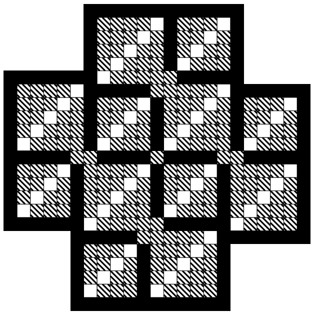

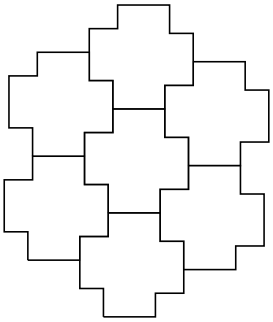

| | | |
|---|---|---|
| $(364, 337+364i)$ | | |
| $(312, 287+312i)$ | $-26i$ | $-13+12i$ |
| $(1, 1+2i)$ | $14+13i$ | $13+1i$ |
| $(1, 1)$ | $-14+13i$ | $-13i$ |
| $(264, 241+264i)$ | | |

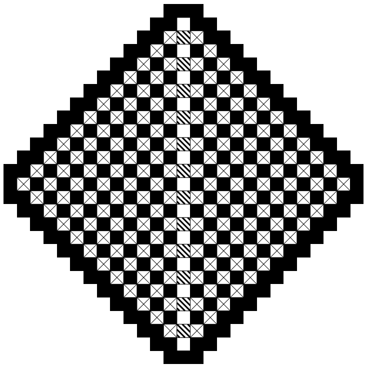

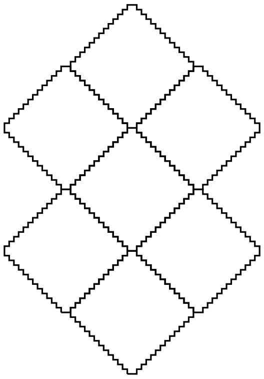

| | | |
|---|---|---|
| $(369, 17+114i)$ | | |
| $(172, 7+52i)$ | $10-21i$ | $-3+2i$ |
| $(36, 1+12i)$ | $9+18i$ | $3+1i$ |
| $(1, 1)$ | $-19+3i$ | $-3i$ |
| $(49, 1+14i)$ | | |

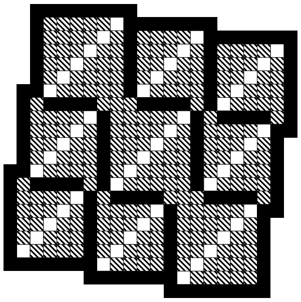
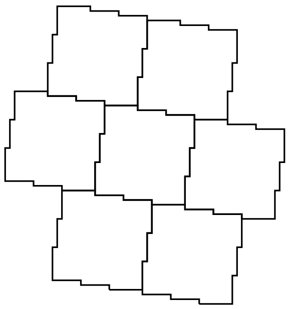

| | | |
|---|---|---|
| $(369, 17+132i)$ | | |
| $(124, 7+44i)$ | $-22+3i$ | $-4i$ |
| $(36, 1+12i)$ | $9-18i$ | $-3+2i$ |
| $(25, 1+10i)$ | $13+15i$ | $3+2i$ |
| $(1, 1)$ | | |

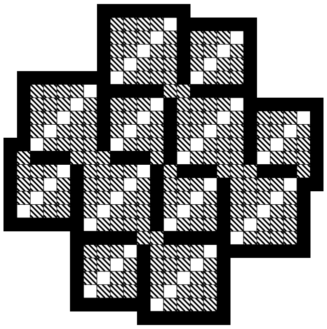
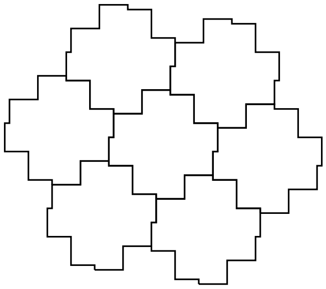

| | | |
|---|---|---|
| $(369, 161+306i)$ | | |
| $(288, 127+240i)$ | $24+9i$ | $9+8i$ |
| $(1, 1)$ | $-17+9i$ | $-9i$ |
| $(4, 1+4i)$ | $-7-18i$ | $-9+1i$ |
| $(217, 97+182i)$ | | |

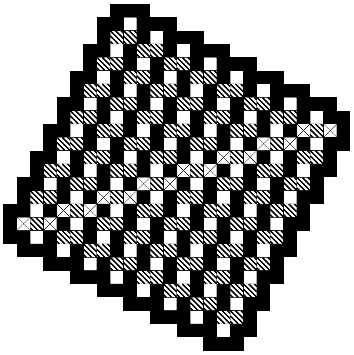
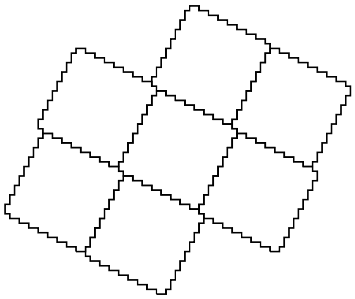

| | | |
|---|---|---|
| $(372, 7+204i)$ | | |
| $(121, 1+66i)$ | $3-22i$ | $-6+1i$ |
| $(49, 1+28i)$ | $15+14i$ | $4+4i$ |
| $(16, 1+8i)$ | $-18+8i$ | $2-5i$ |
| $(0, -1)$ | | |

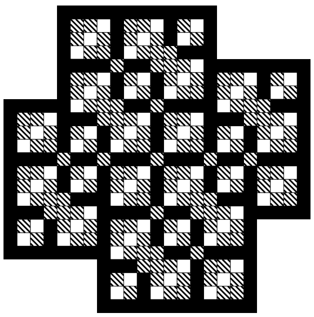
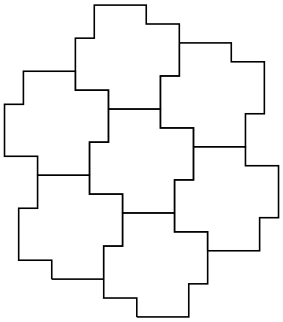

| | | |
|---|---|---|
| $(372, 97+252i)$ | | |
| $(193, 49+130i)$ | $6-23i$ | $-7+5i$ |
| $(28, 7+20i)$ | $12+16i$ | $7+2i$ |
| $(1, 1)$ | $-18+7i$ | $-7i$ |
| $(72, 17+48i)$ | | |

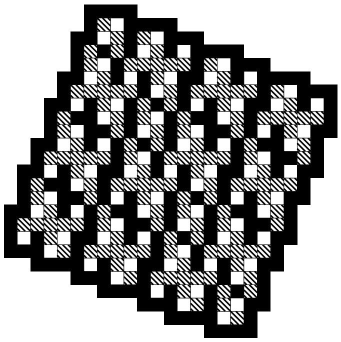
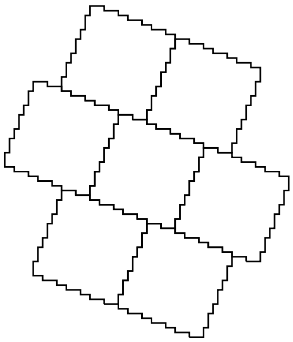

| | | |
|---|---|---|
| $(376, 31+152i)$ | | |
| $(204, 17+84i)$ | $18+16i$ | $4+3i$ |
| $(1, 1)$ | $-19+4i$ | $-4i$ |
| $(25, 1+10i)$ | $1-20i$ | $-4+1i$ |
| $(84, 7+36i)$ | | |

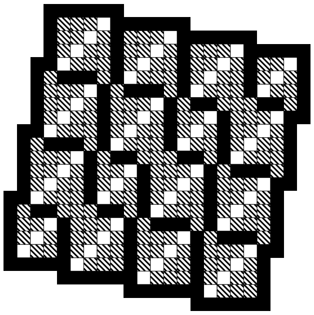
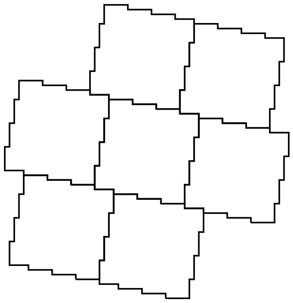

| | | |
|---|---|---|
| $(376, 241+352i)$ | | |
| $(249, 161+234i)$ | $24+7i$ | $11+9i$ |
| $(1, 1)$ | $-16+11i$ | $-11i$ |
| $(12, 7+12i)$ | $-8-18i$ | $-11+2i$ |
| $(148, 97+140i)$ | | |

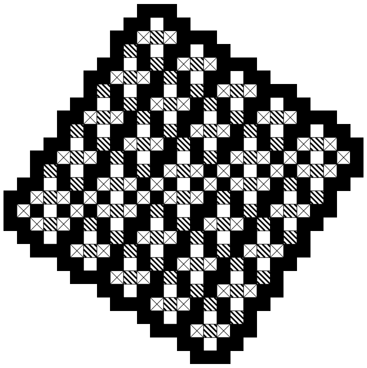
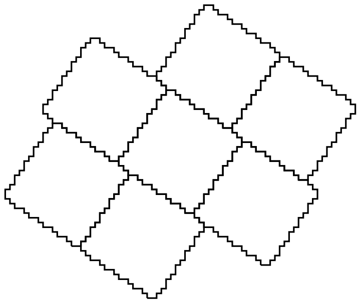

| | | |
|---|---|---|
| $(384, 31+312i)$ | | |
| $(201, 17+162i)$ | $-21+12i$ | $4-9i$ |
| $(25, 1+20i)$ | $3-20i$ | $-8+2i$ |
| $(4, 1+4i)$ | $18+8i$ | $4+7i$ |
| $(76, 7+60i)$ | | |

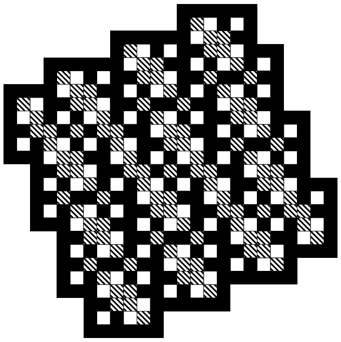
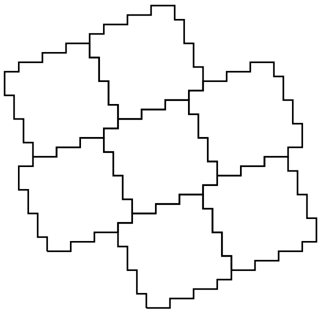

| | | |
|---|---|---|
| $(385, 49+190i)$ | | |
| $(240, 31+120i)$ | $20+15i$ | $5+4i$ |
| $(1, 1)$ | $-19+5i$ | $-5i$ |
| $(16, 1+8i)$ | $-1-20i$ | $-5+1i$ |
| $(129, 17+66i)$ | | |

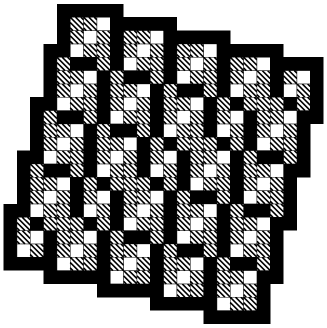
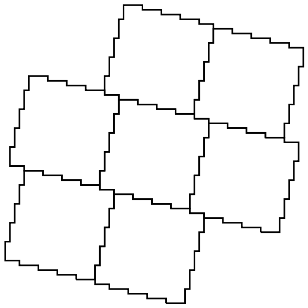

| | | |
|---|---|---|
| $(385, 49+300i)$ | | |
| $(256, 31+200i)$ | $-4-25i$ | $-10$ |
| $(4, 1+4i)$ | $17+10i$ | $5+6i$ |
| $(9, 1+6i)$ | $-13+15i$ | $5-6i$ |
| $(153, 17+120i)$ | | |

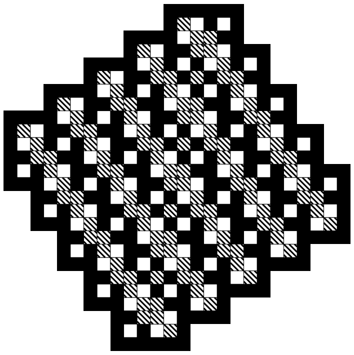

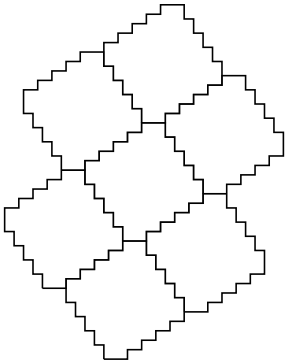

| | | |
|---|---|---|
| $(385, 289+380i)$ | | |
| $(129, 97+126i)$ | $-17+15i$ | $1-14i$ |
| $(24, 17+24i)$ | $-3-20i$ | $-11+6i$ |
| $(40, 31+40i)$ | $20+5i$ | $10+8i$ |
| $(1, 1)$ | | |

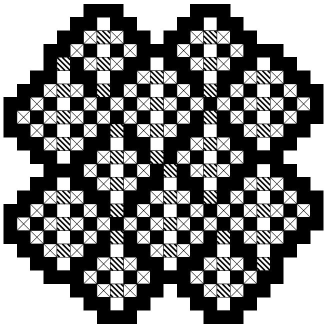

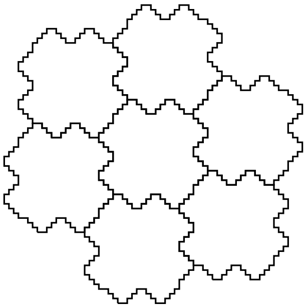

| | | |
|---|---|---|
| $(388, 7+284i)$ | | |
| $(121, 1+88i)$ | $5-22i$ | $-8+2i$ |
| $(64, 1+48i)$ | $14+16i$ | $6+5i$ |
| $(9, 1+6i)$ | $-19+6i$ | $2-7i$ |
| $(0, -1)$ | | |

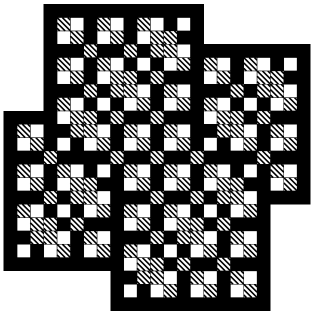

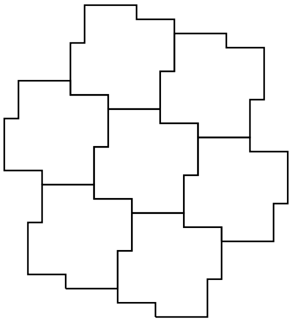

| | | |
|---|---|---|
| $(388, 199+340i)$ | | |
| $(192, 97+168i)$ | $2-24i$ | $-10+7i$ |
| $(33, 17+30i)$ | $15+14i$ | $10+3i$ |
| $(1, 1)$ | $-17+10i$ | $-10i$ |
| $(64, 31+56i)$ | | |

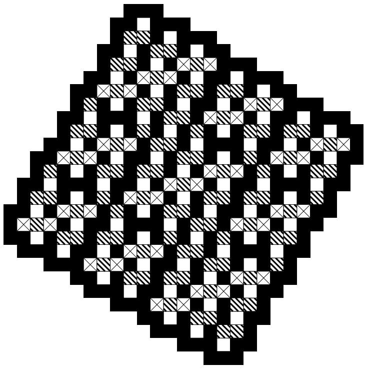

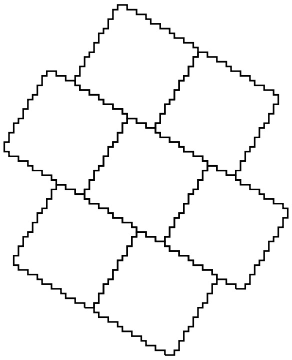

| | | |
|---|---|---|
| $(393, 49+204i)$ | | |
| $(129, 17+66i)$ | $-21+9i$ | $1-6i$ |
| $(16, 1+8i)$ | $3-20i$ | $-5+2i$ |
| $(52, 7+28i)$ | $18+11i$ | $4+4i$ |
| $(1, 1)$ | | |

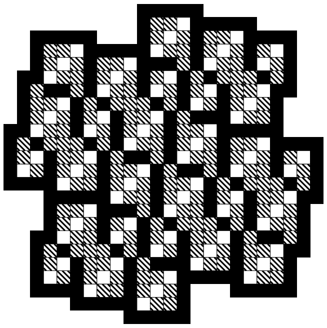

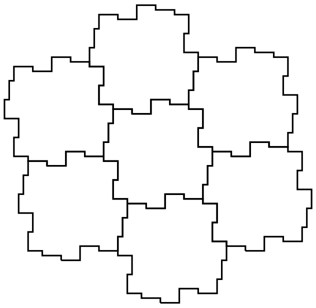

| | | |
|---|---|---|
| $(393, 17+336i)$ | | |
| $(156, 7+132i)$ | $-18+15i$ | $6-8i$ |
| $(49, 1+42i)$ | $-1-21i$ | $-9$ |
| $(4, 1+4i)$ | $19+6i$ | $3+8i$ |
| $(25, 1+20i)$ | | |

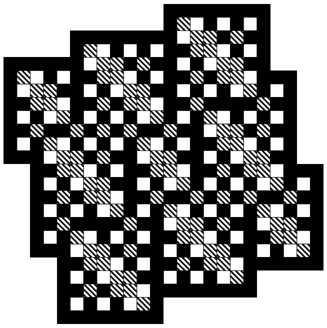

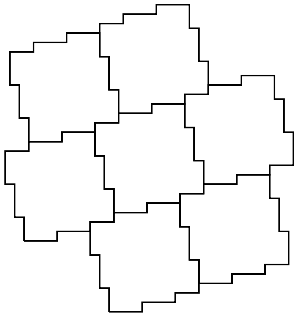

| | | |
|---|---|---|
| $(393, 337+390i)$ | | |
| $(112, 97+112i)$ | $21+8i$ | $13+7i$ |
| $(1, 1)$ | $-15+13i$ | $-13i$ |
| $(84, 71+84i)$ | $-6-21i$ | $-13+6i$ |
| $(1, 1+2i)$ | | |

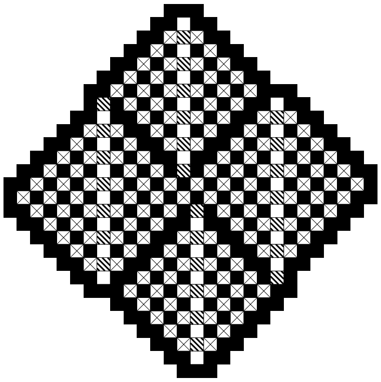

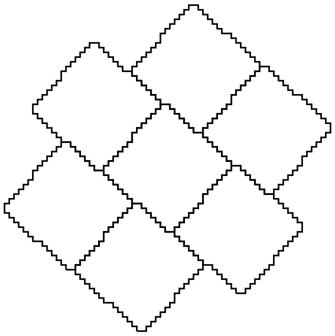

| | | |
|---|---|---|
| $(396, 17+228i)$ | | |
| $(148, 7+84i)$ | $-20+12i$ | $3-6i$ |
| $(49, 1+28i)$ | $2-21i$ | $-6+1i$ |
| $(9, 1+6i)$ | $18+9i$ | $3+5i$ |
| $(16, 1+8i)$ | | |

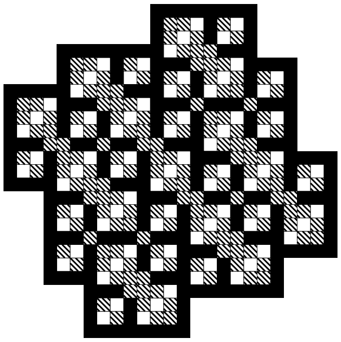

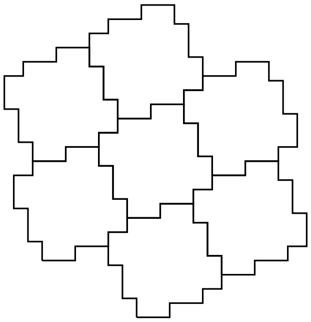

| | | |
|---|---|---|
| $(396, 71+228i)$ | | |
| $(280, 49+160i)$ | $10-24i$ | $-6+5i$ |
| $(9, 1+6i)$ | $9+18i$ | $6+1i$ |
| $(1, 1)$ | $-19+6i$ | $-6i$ |
| $(184, 31+104i)$ | | |

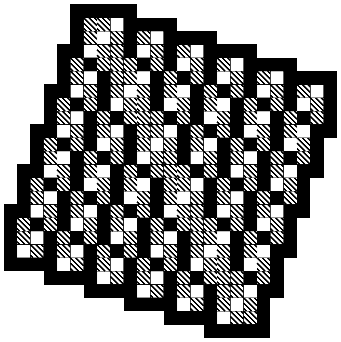
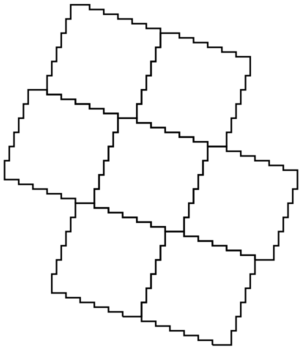

| | | |
|---|---|---|
| $(396, 17+300i)$ | | |
| $(196, 7+148i)$ | $4-24i$ | $-9+2i$ |
| $(25, 1+20i)$ | $14+15i$ | $6+5i$ |
| $(9, 1+6i)$ | $-18+9i$ | $3-7i$ |
| $(64, 1+48i)$ | | |

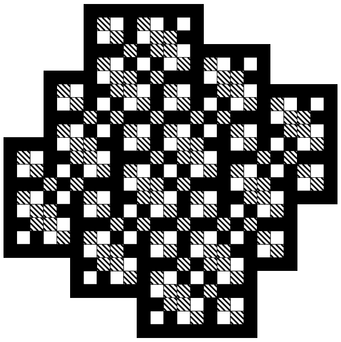
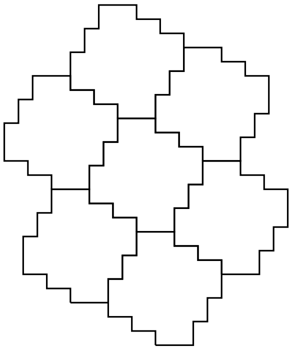

| | | |
|---|---|---|
| $(396, 71+300i)$ | | |
| $(265, 49+200i)$ | $-25+6i$ | $-10i$ |
| $(9, 1+6i)$ | $9-18i$ | $-6+5i$ |
| $(4, 1+4i)$ | $16+12i$ | $6+5i$ |
| $(160, 31+120i)$ | | |

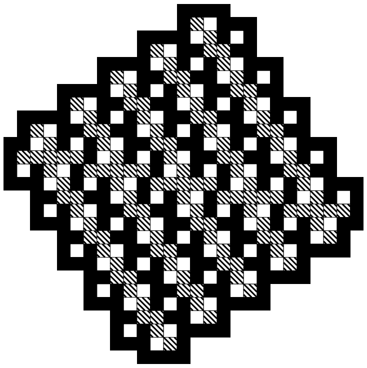
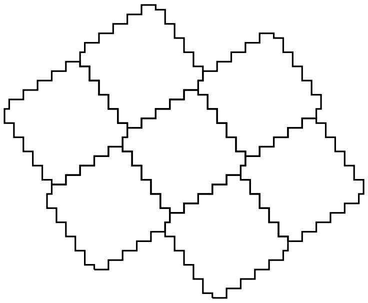

| | | |
|---|---|---|
| $(400, 1+40i)$ | | |
| $(361, 1+38i)$ | $20+19i$ | $1+1i$ |
| $(1, 1)$ | $-20+1i$ | $-1i$ |
| $(0, -1)$ | $-20i$ | $-1$ |
| $(324, 1+36i)$ | | |

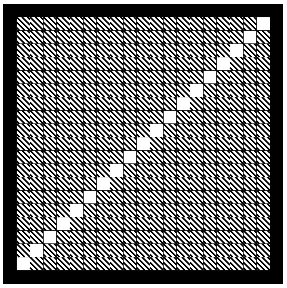
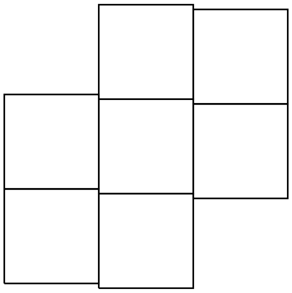

| | | |
|---|---|---|
| $(400, 1+120i)$ | | |
| $(169, 1+52i)$ | $20+13i$ | $2+3i$ |
| $(49, 1+14i)$ | $-20+7i$ | $1-3i$ |
| $(0, -1)$ | $-20i$ | $-3$ |
| $(36, 1+12i)$ | | |

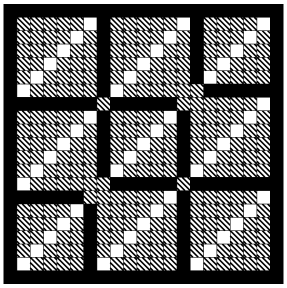
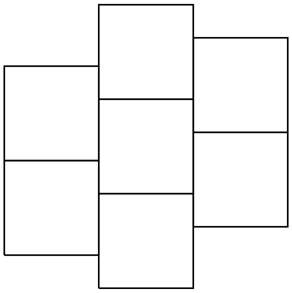

| | | |
|---|---|---|
| $(400, 1+280i)$ | | |
| $(289, 1+204i)$ | $20+17i$ | $6+7i$ |
| $(9, 1+6i)$ | $-20+3i$ | $1-7i$ |
| $(0, -1)$ | $-20i$ | $-7$ |
| $(196, 1+140i)$ | | |

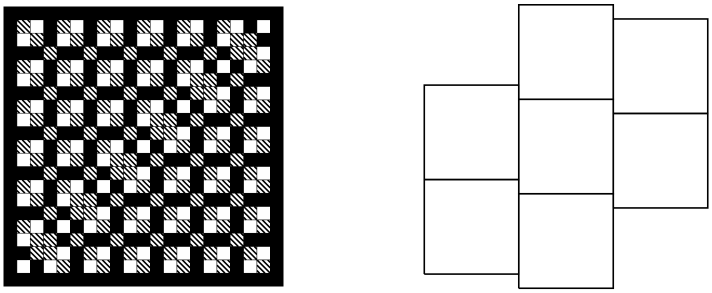

| | | |
|---|---|---|
| $(400, 1+360i)$ | | |
| $(121, 1+110i)$ | $20+11i$ | $5+9i$ |
| $(81, 1+72i)$ | $-20+9i$ | $4-9i$ |
| $(0, -1)$ | $-20i$ | $-9$ |
| $(4, 1+4i)$ | | |

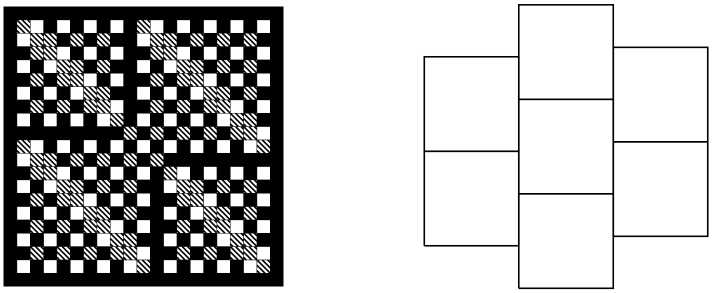

| | | |
|---|---|---|
| $(408, 17+120i)$ | | |
| $(172, 7+52i)$ | $16+18i$ | $3+2i$ |
| $(1, 1)$ | $-20+3i$ | $-3i$ |
| $(49, 1+14i)$ | $4-21i$ | $-3+1i$ |
| $(36, 1+12i)$ | | |

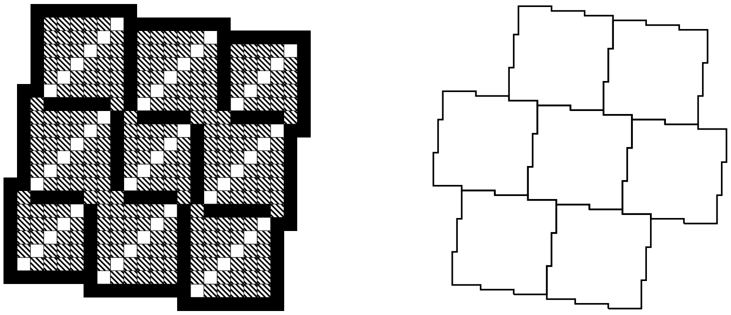

| | | |
|---|---|---|
| $(409, 97+266i)$ | | |
| $(136, 31+88i)$ | $4-23i$ | $-7+4i$ |
| $(72, 17+48i)$ | $15+16i$ | $7+3i$ |
| $(1, 1)$ | $-19+7i$ | $-7i$ |
| $(9, 1+6i)$ | | |

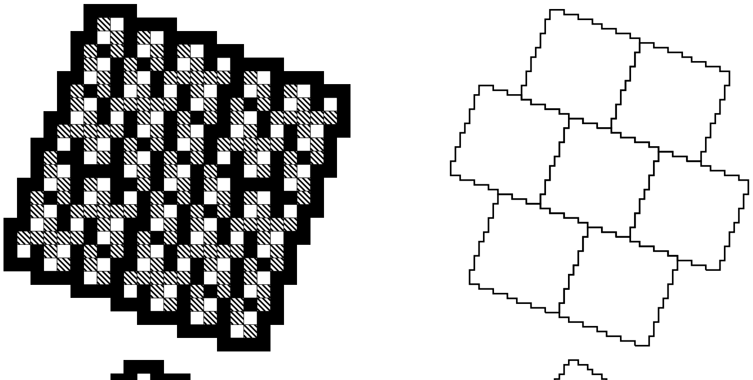

| | | |
|---|---|---|
| $(409, 241+374i)$ | | |
| $(276, 161+252i)$ | $3-26i$ | $-11+9i$ |
| $(12, 7+12i)$ | $14+15i$ | $11+2i$ |
| $(1, 1)$ | $-17+11i$ | $-11i$ |
| $(169, 97+154i)$ | | |

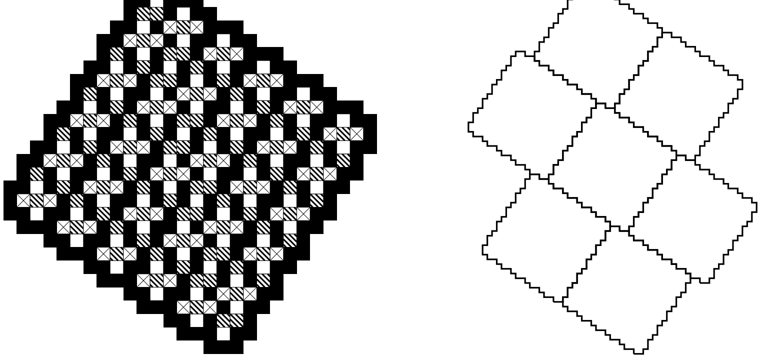

| | | |
|---|---|---|
| $(412, 49+228i)$ | | |
| $(153, 17+84i)$ | $6-23i$ | $-6+3i$ |
| $(9, 1+6i)$ | $14+15i$ | $5+3i$ |
| $(52, 7+28i)$ | $-20+8i$ | $1-6i$ |
| $(16, 1+8i)$ | | |

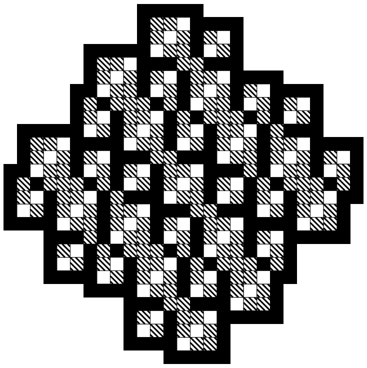

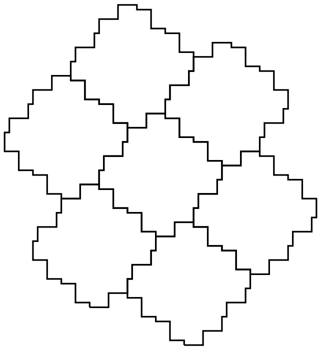

| | | |
|---|---|---|
| $(412, 7+372i)$ | | |
| $(121, 1+110i)$ | $-7-22i$ | $-10-3i$ |
| $(4, 1+4i)$ | $20+4i$ | $2+9i$ |
| $(81, 1+72i)$ | $-13+18i$ | $8-6i$ |
| $(0, -1)$ | | |

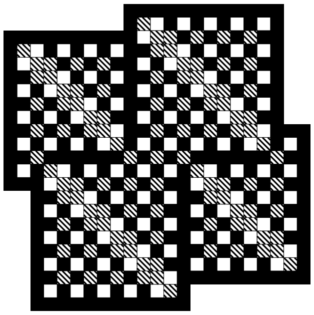

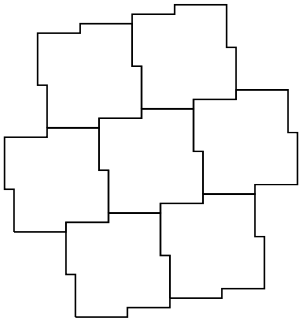

| | | |
|---|---|---|
| $(412, 199+372i)$ | | |
| $(201, 97+180i)$ | $-17+18i$ | $4-12i$ |
| $(4, 1+4i)$ | $-4-20i$ | $-10+3i$ |
| $(33, 17+30i)$ | $21+2i$ | $6+9i$ |
| $(64, 31+56i)$ | | |

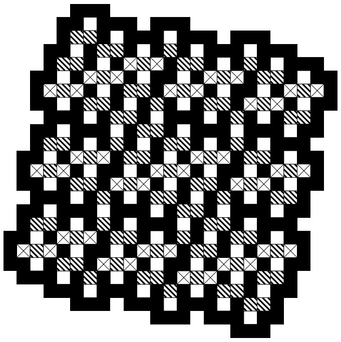

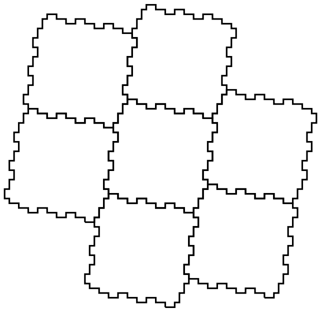

| | | |
|---|---|---|
| $(417, 17+234i)$ | | |
| $(148, 7+84i)$ | $22+9i$ | $3+6i$ |
| $(16, 1+8i)$ | $-17+12i$ | $3-5i$ |
| $(49, 1+28i)$ | $-5-21i$ | $-6-1i$ |
| $(9, 1+6i)$ | | |

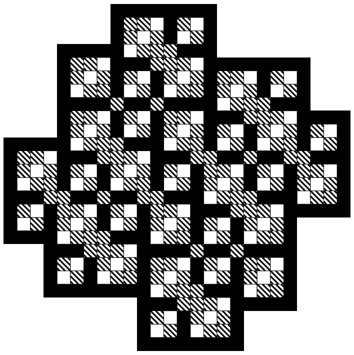

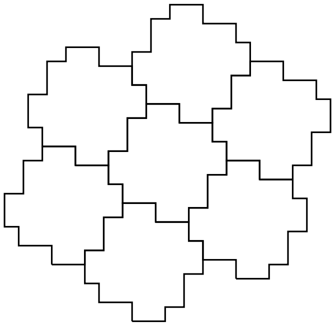

| | | |
|---|---|---|
| $(417, 97+312i)$ | | |
| $(217, 49+162i)$ | $3-25i$ | $-9+4i$ |
| $(4, 1+4i)$ | $15+14i$ | $7+4i$ |
| $(28, 7+20i)$ | $-18+11i$ | $2-8i$ |
| $(81, 17+60i)$ | | |

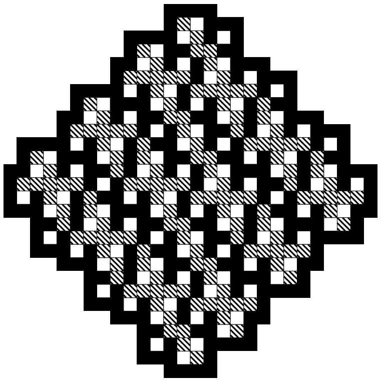
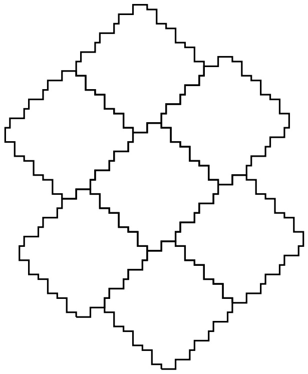

| | | |
|---|---|---|
| $(420, 391+420i)$ | | |
| $(364, 337+364i)$ | $-28i$ | $-14+13i$ |
| $(1, 1+2i)$ | $15+14i$ | $14+1i$ |
| $(1, 1)$ | $-15+14i$ | $-14i$ |
| $(312, 287+312i)$ | | |

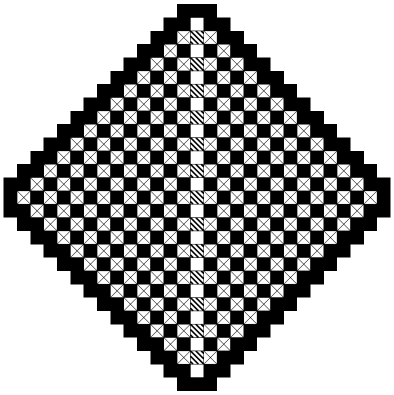
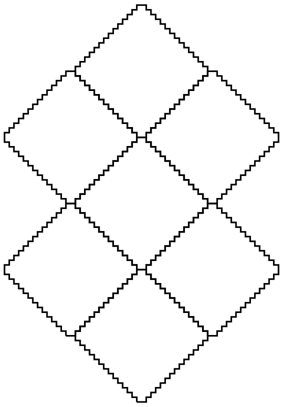

| | | |
|---|---|---|
| $(424, 31+328i)$ | | |
| $(216, 17+168i)$ | $24+8i$ | $4+9i$ |
| $(9, 1+6i)$ | $-17+12i$ | $4-7i$ |
| $(25, 1+20i)$ | $-7-20i$ | $-8-2i$ |
| $(76, 7+60i)$ | | |

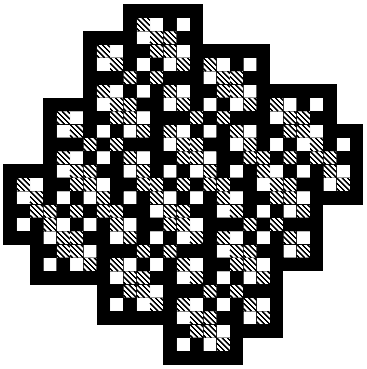
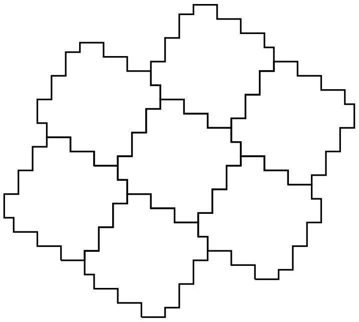

| | | |
|---|---|---|
| $(424, 127+304i)$ | | |
| $(168, 49+120i)$ | $4-24i$ | $-8+5i$ |
| $(57, 17+42i)$ | $15+16i$ | $8+3i$ |
| $(1, 1)$ | $-19+8i$ | $-8i$ |
| $(28, 7+20i)$ | | |

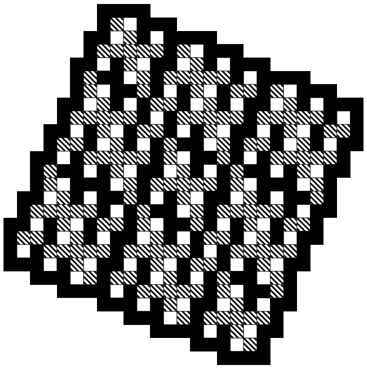
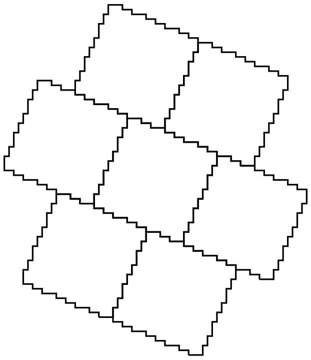

| | | |
|---|---|---|
| $(424, 337+416i)$ | | |
| $(201, 161+198i)$ | $24+7i$ | $13+9i$ |
| $(1,1)$ | $-16+13i$ | $-13i$ |
| $(40, 31+40i)$ | $-8-20i$ | $-13+4i$ |
| $(60, 49+60i)$ | | |

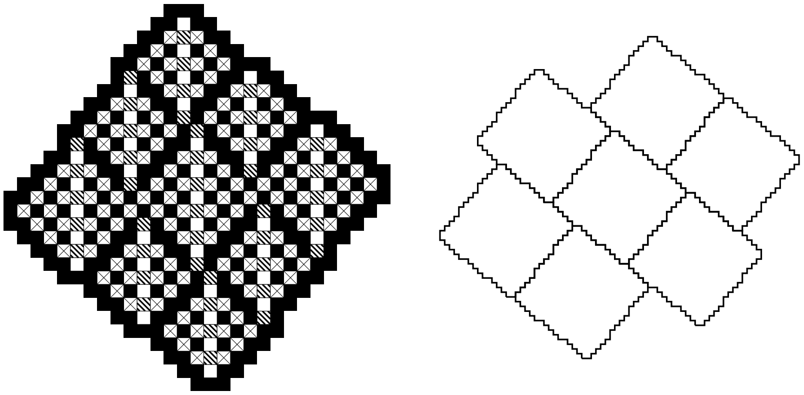

| | | |
|---|---|---|
| $(432, 287+408i)$ | | |
| $(148, 97+140i)$ | $-2-24i$ | $-12+7i$ |
| $(73, 49+70i)$ | $19+12i$ | $12+5i$ |
| $(1,1)$ | $-17+12i$ | $-12i$ |
| $(12, 7+12i)$ | | |

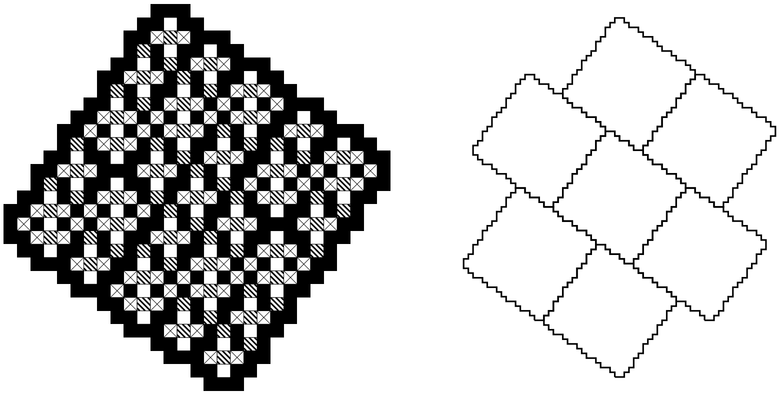

| | | |
|---|---|---|
| $(433, 49+234i)$ | | |
| $(153, 17+84i)$ | $15+19i$ | $6+3i$ |
| $(52, 7+28i)$ | $-22+1i$ | $-1-6i$ |
| $(16, 1+8i)$ | $7-20i$ | $-5+3i$ |
| $(9, 1+6i)$ | | |

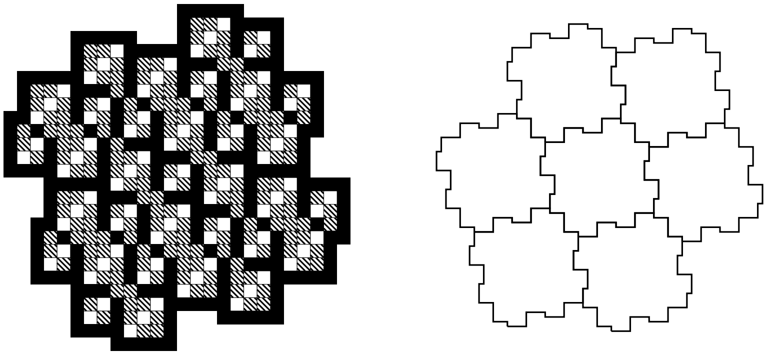

| | | |
|---|---|---|
| $(433, 97+284i)$ | | |
| $(136, 31+88i)$ | $-20+13i$ | $2-8i$ |
| $(9, 1+6i)$ | $-1-21i$ | $-7+2i$ |
| $(72, 17+48i)$ | $21+8i$ | $5+6i$ |
| $(1,1)$ | | |

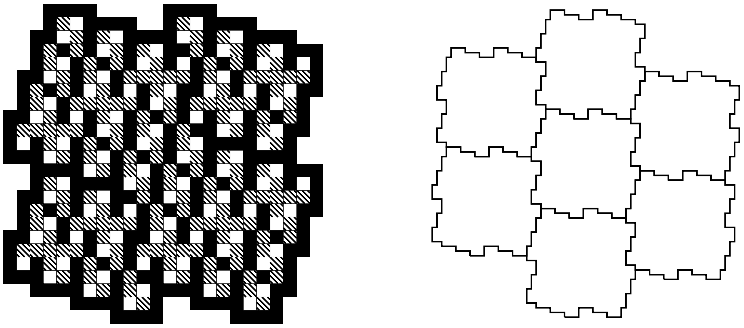

| | | |
|---|---|---|
| $(433, 289 + 426i)$ | | |
| $(217, 145 + 212i)$ | $-19 + 17i$ | $2 - 15i$ |
| $(12, 7 + 12i)$ | $-2 - 21i$ | $-11 + 6i$ |
| $(24, 17 + 24i)$ | $21 + 4i$ | $9 + 9i$ |
| $(73, 49 + 70i)$ | | |

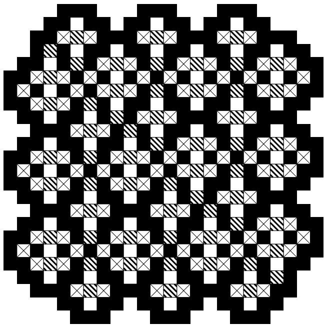
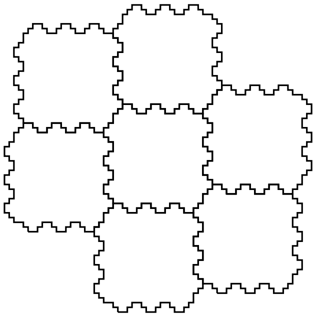

| | | |
|---|---|---|
| $(436, 97 + 300i)$ | | |
| $(217, 49 + 148i)$ | $-22 + 13i$ | $2 - 9i$ |
| $(9, 1 + 6i)$ | $2 - 21i$ | $-7 + 3i$ |
| $(28, 7 + 20i)$ | $20 + 8i$ | $5 + 6i$ |
| $(72, 17 + 48i)$ | | |

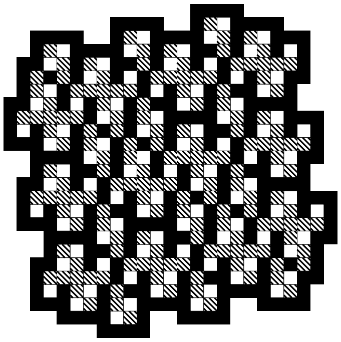
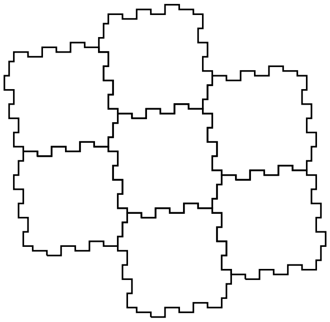

| | | |
|---|---|---|
| $(436, 7 + 364i)$ | | |
| $(144, 1 + 120i)$ | $2 - 24i$ | $-10 + 1i$ |
| $(49, 1 + 42i)$ | $17 + 14i$ | $6 + 7i$ |
| $(25, 1 + 20i)$ | $-19 + 10i$ | $4 - 8i$ |
| $(0, -1)$ | | |

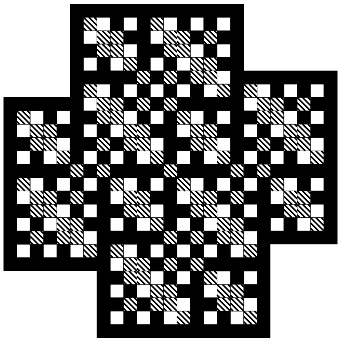
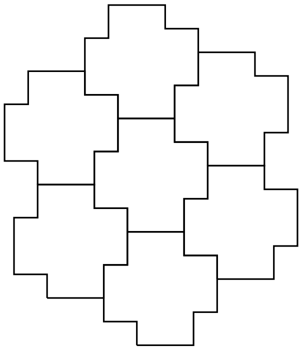

| | | |
|---|---|---|
| $(441, 1 + 42i)$ | | |
| $(400, 1 + 40i)$ | $21 + 20i$ | $1 + 1i$ |
| $(1, 1)$ | $-21 + 1i$ | $-1i$ |
| $(0, -1)$ | $-21i$ | $-1$ |
| $(361, 1 + 38i)$ | | |

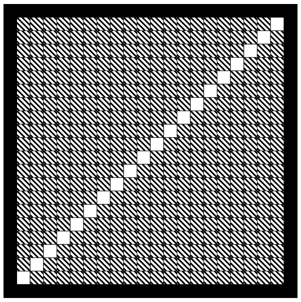
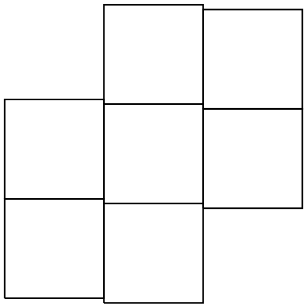

| | | |
|---|---|---|
| $(441, 1 + 84i)$ | | |
| $(121, 1 + 22i)$ | $-21 + 11i$ | $1 - 2i$ |
| $(0, -1)$ | $-21i$ | $-2$ |
| $(100, 1 + 20i)$ | $21 + 10i$ | $1 + 2i$ |
| $(1, 1)$ | | |

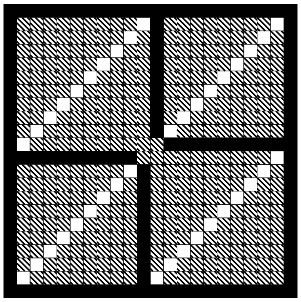
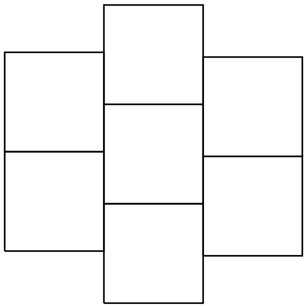

| | | |
|---|---|---|
| $(441, 1+168i)$ | | |
| $(256, 1+96i)$ | $-21+16i$ | $3-4i$ |
| $(0, -1)$ | $-21i$ | $-4$ |
| $(25, 1+10i)$ | $21+5i$ | $1+4i$ |
| $(121, 1+44i)$ | | |

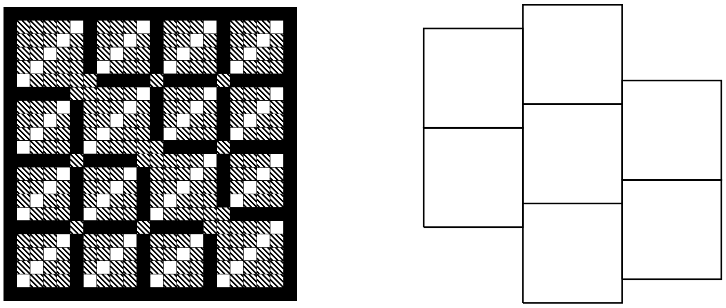

| | | |
|---|---|---|
| $(441, 1+210i)$ | | |
| $(289, 1+136i)$ | $-21+17i$ | $4-5i$ |
| $(0, -1)$ | $-21i$ | $-5$ |
| $(16, 1+8i)$ | $21+4i$ | $1+5i$ |
| $(169, 1+78i)$ | | |

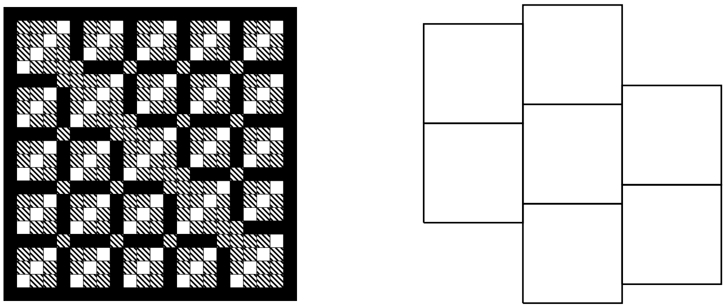

| | | |
|---|---|---|
| $(441, 1+336i)$ | | |
| $(169, 1+130i)$ | $21+13i$ | $5+8i$ |
| $(64, 1+48i)$ | $-21+8i$ | $3-8i$ |
| $(0, -1)$ | $-21i$ | $-8$ |
| $(25, 1+20i)$ | | |

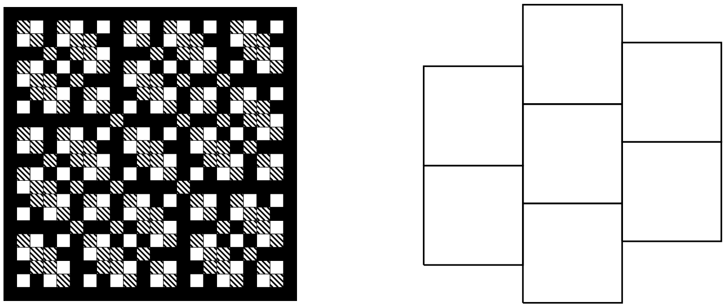

| | | |
|---|---|---|
| $(441, 161+342i)$ | | |
| $(352, 127+272i)$ | $8-27i$ | $-9+8i$ |
| $(4, 1+4i)$ | $11+18i$ | $9+1i$ |
| $(1, 1)$ | $-19+9i$ | $-9i$ |
| $(273, 97+210i)$ | | |

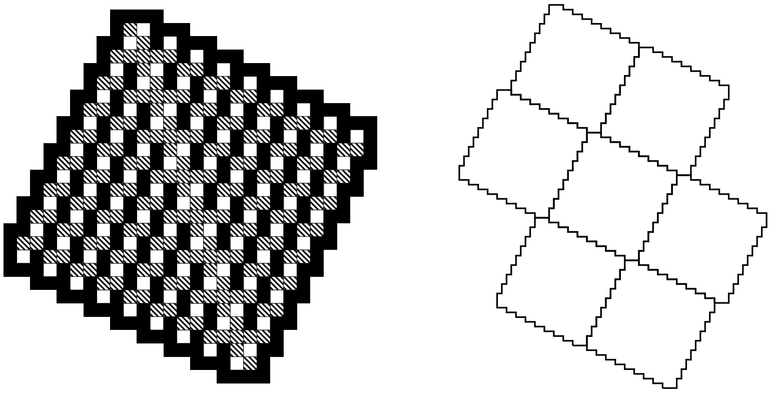

| | | |
|---|---|---|
| $(441, 1+420i)$ | | |
| $(361, 1+342i)$ | $-21+19i$ | $9-10i$ |
| $(0, -1)$ | $-21i$ | $-10$ |
| $(4, 1+4i)$ | $21+2i$ | $1+10i$ |
| $(289, 1+272i)$ | | |

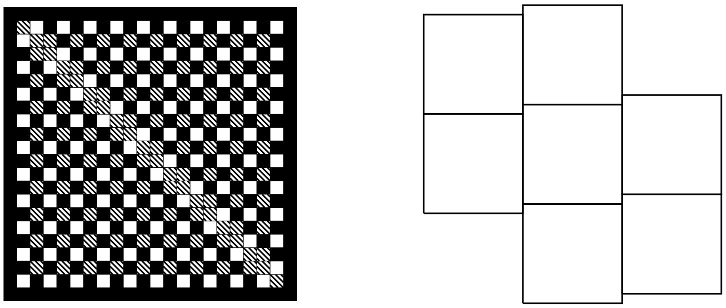

| | | |
|---|---|---|
| $(444, 7+84i)$ | | |
| $(121, 1+22i)$ | $9-22i$ | $-2+1i$ |
| $(100, 1+20i)$ | $12+20i$ | $2+1i$ |
| $(1, 1)$ | $-21+2i$ | $-2i$ |
| $(0, -1)$ | | |

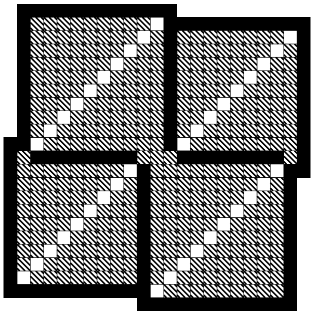

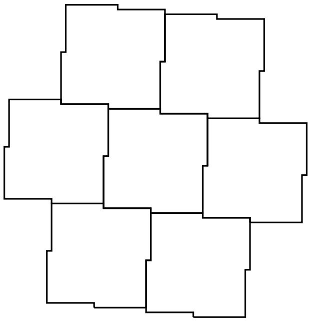

| | | |
|---|---|---|
| $(444, 241+396i)$ | | |
| $(232, 127+208i)$ | $24+10i$ | $11+8i$ |
| $(1, 1)$ | $-18+11i$ | $-11i$ |
| $(33, 17+30i)$ | $-6-21i$ | $-11+3i$ |
| $(88, 49+80i)$ | | |

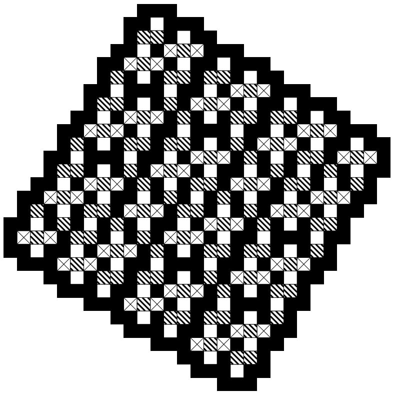

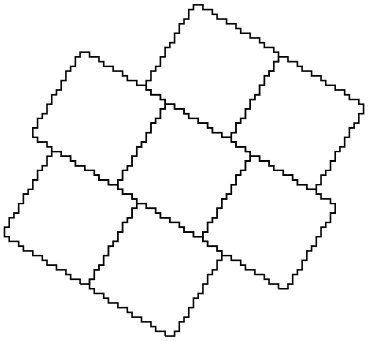

| | | |
|---|---|---|
| $(448, 97+280i)$ | | |
| $(324, 71+204i)$ | $24+14i$ | $7+6i$ |
| $(1, 1)$ | $-20+7i$ | $-7i$ |
| $(9, 1+6i)$ | $-4-21i$ | $-7+1i$ |
| $(220, 49+140i)$ | | |

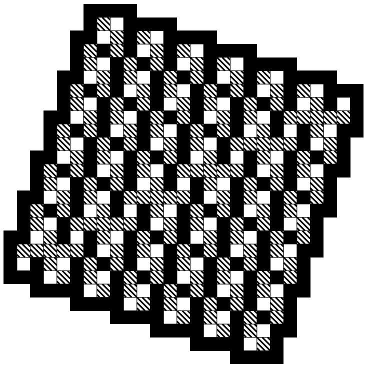

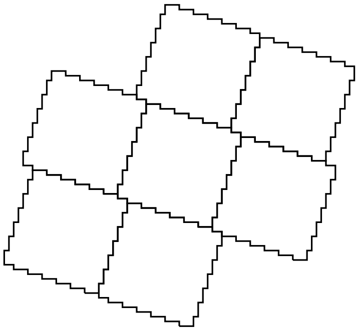

| | | |
|---|---|---|
| $(448, 127+336i)$ | | |
| $(177, 49+132i)$ | $7-24i$ | $-8+6i$ |
| $(4, 1+4i)$ | $14+16i$ | $8+3i$ |
| $(57, 17+42i)$ | $-21+8i$ | $-9i$ |
| $(28, 7+20i)$ | | |

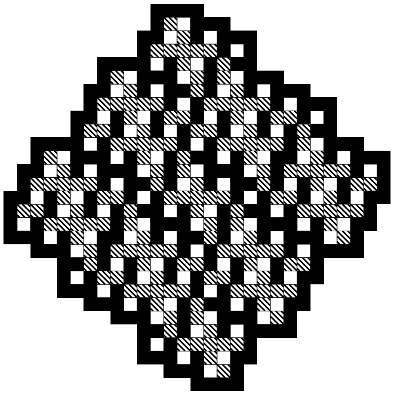

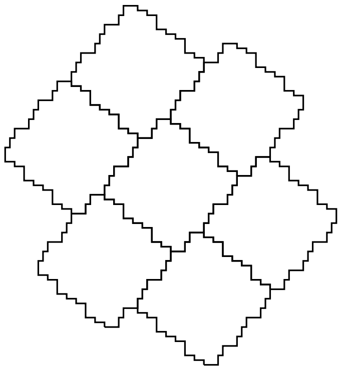

| | | |
|---|---|---|
| $(456, 31 + 168i)$ | | |
| $(264, 17 + 96i)$ | $12 - 24i$ | $-4 + 3i$ |
| $(25, 1 + 10i)$ | $9 + 20i$ | $4 + 1i$ |
| $(1, 1)$ | $-21 + 4i$ | $-4i$ |
| $(124, 7 + 44i)$ | | |

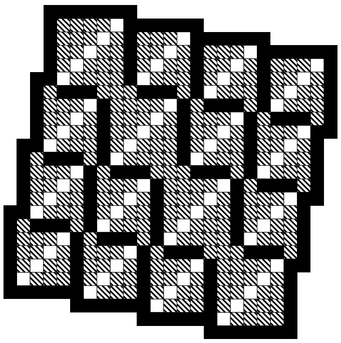
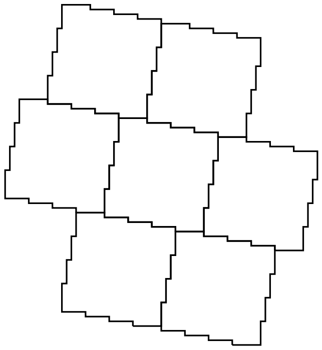

| | | |
|---|---|---|
| $(456, 17 + 384i)$ | | |
| $(156, 7 + 132i)$ | $24 + 6i$ | $3 + 10i$ |
| $(25, 1 + 20i)$ | $-16 + 15i$ | $6 - 7i$ |
| $(49, 1 + 42i)$ | $-8 - 21i$ | $-9 - 3i$ |
| $(4, 1 + 4i)$ | | |

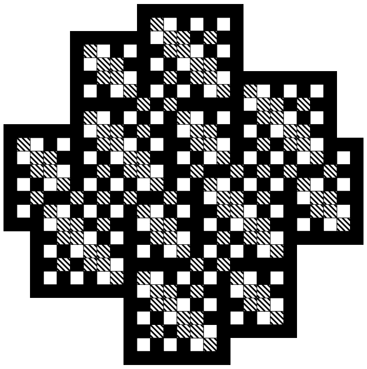
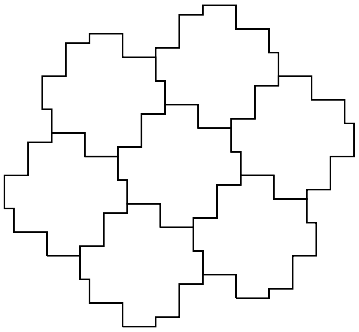

| | | |
|---|---|---|
| $(457, 97 + 328i)$ | | |
| $(232, 49 + 168i)$ | $17 + 20i$ | $9 + 4i$ |
| $(28, 7 + 20i)$ | $-22 + 1i$ | $-2 - 8i$ |
| $(9, 1 + 6i)$ | $5 - 21i$ | $-7 + 4i$ |
| $(81, 17 + 60i)$ | | |

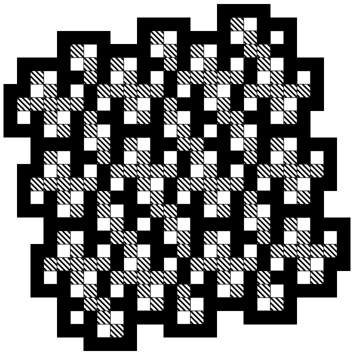
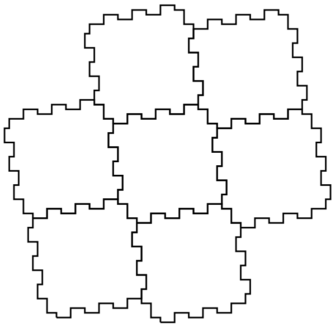

| | | |
|---|---|---|
| $(457, 49 + 362i)$ | | |
| $(153, 17 + 120i)$ | $-21 + 13i$ | $4 - 9i$ |
| $(76, 7 + 60i)$ | $2 - 23i$ | $-9 + 2i$ |
| $(4, 1 + 4i)$ | $19 + 10i$ | $5 + 7i$ |
| $(9, 1 + 6i)$ | | |

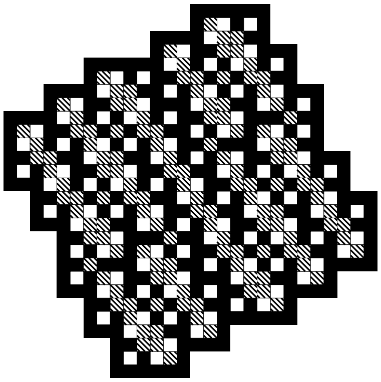
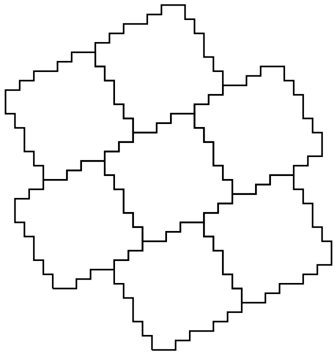

| | | |
|---|---|---|
| $(457, 337 + 442i)$ | | |
| $(268, 199 + 260i)$ | $26 + 7i$ | $13 + 10i$ |
| $(1, 1)$ | $-17 + 13i$ | $-13i$ |
| $(24, 17 + 24i)$ | $-9 - 20i$ | $-13 + 3i$ |
| $(129, 97 + 126i)$ | | |

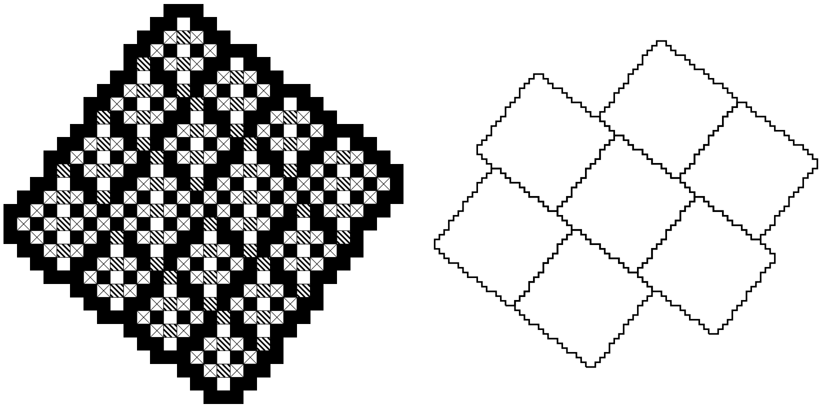

| | | |
|---|---|---|
| $(460, 199 + 380i)$ | | |
| $(369, 161 + 306i)$ | $27 + 10i$ | $10 + 9i$ |
| $(1, 1)$ | $-19 + 10i$ | $-10i$ |
| $(4, 1 + 4i)$ | $-8 - 20i$ | $-10 + 1i$ |
| $(288, 127 + 240i)$ | | |

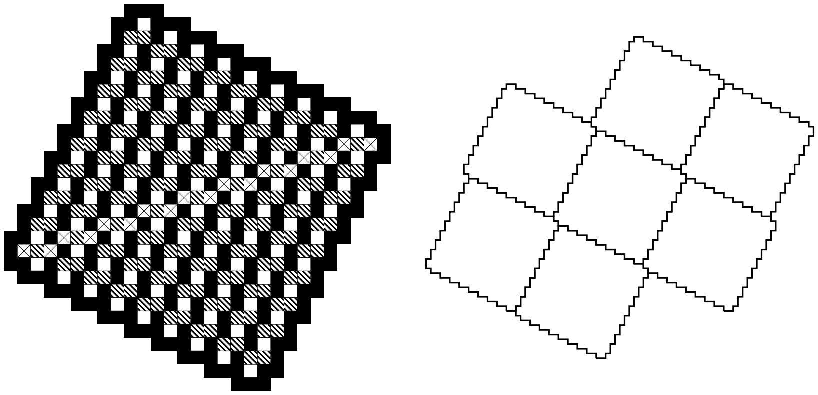

| | | |
|---|---|---|
| $(465, 49 + 210i)$ | | |
| $(304, 31 + 136i)$ | $12 - 25i$ | $-5 + 4i$ |
| $(16, 1 + 8i)$ | $9 + 20i$ | $5 + 1i$ |
| $(1, 1)$ | $-21 + 5i$ | $-5i$ |
| $(177, 17 + 78i)$ | | |

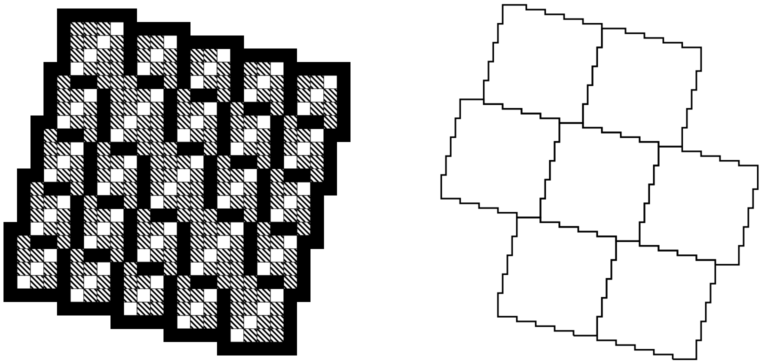

| | | |
|---|---|---|
| $(465, 305 + 444i)$ | | |
| $(148, 97 + 140i)$ | $-17 + 18i$ | $3 - 14i$ |
| $(12, 7 + 12i)$ | $-6 - 21i$ | $-12 + 4i$ |
| $(73, 49 + 70i)$ | $23 + 3i$ | $9 + 10i$ |
| $(1, 1)$ | | |

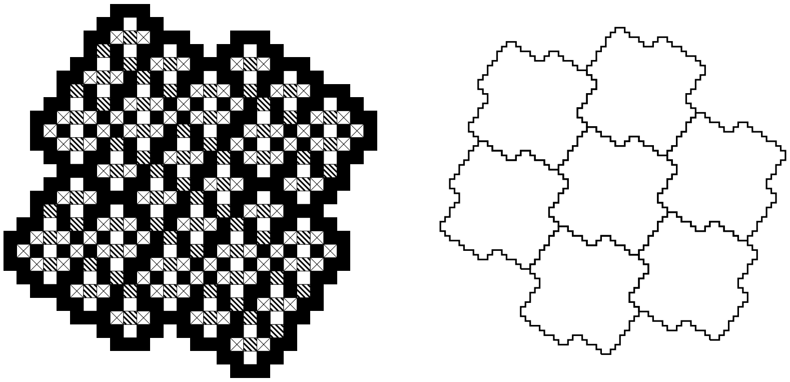

| | | |
|---|---|---|
| $(472, 49+368i)$ | | |
| $(153, 17+120i)$ | $24+7i$ | $4+9i$ |
| $(9, 1+6i)$ | $-16+15i$ | $5-7i$ |
| $(76, 7+60i)$ | $-8-22i$ | $-9-2i$ |
| $(4, 1+4i)$ | | |

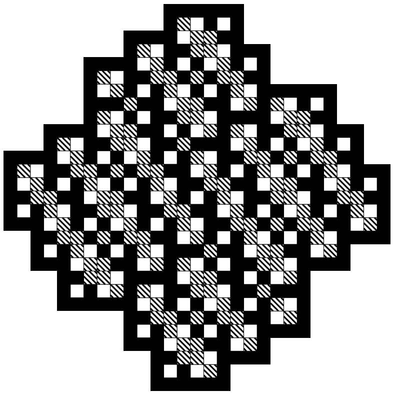
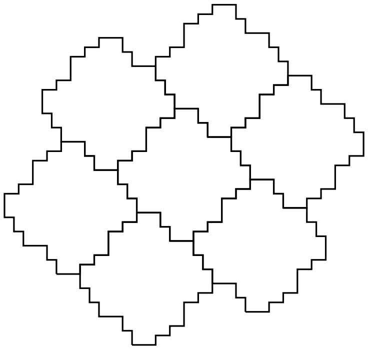

| | | |
|---|---|---|
| $(480, 161+360i)$ | | |
| $(145, 49+110i)$ | $20+15i$ | $9+5i$ |
| $(1, 1)$ | $-20+9i$ | $-9i$ |
| $(96, 31+72i)$ | $-24i$ | $-9+4i$ |
| $(4, 1+4i)$ | | |

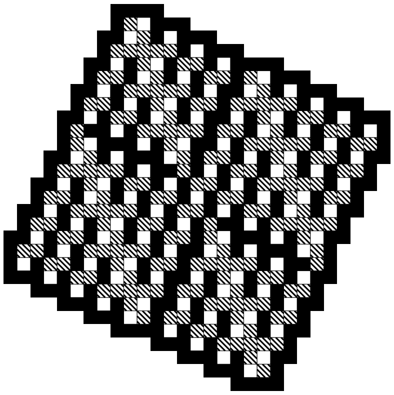
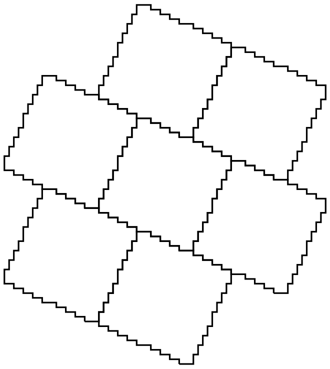

| | | |
|---|---|---|
| $(480, 449+480i)$ | | |
| $(420, 391+420i)$ | $-30i$ | $-15+14i$ |
| $(1, 1+2i)$ | $16+15i$ | $15+1i$ |
| $(1, 1)$ | $-16+15i$ | $-15i$ |
| $(364, 337+364i)$ | | |

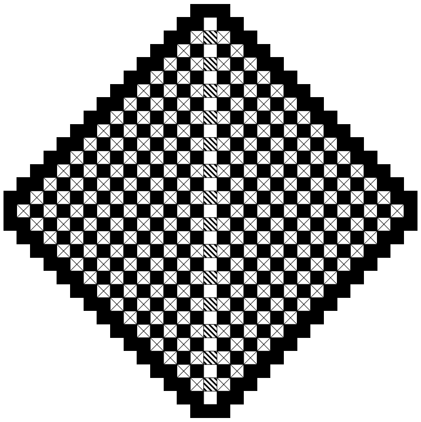
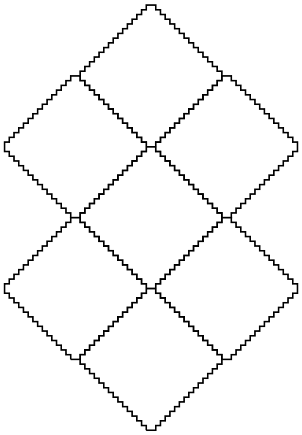

| | | |
|---|---|---|
| $(481, 97+362i)$ | | |
| $(160, 31+120i)$ | $4-25i$ | $-9+4i$ |
| $(4, 1+4i)$ | $17+14i$ | $7+5i$ |
| $(81, 17+60i)$ | $-21+11i$ | $2-9i$ |
| $(9, 1+6i)$ | | |

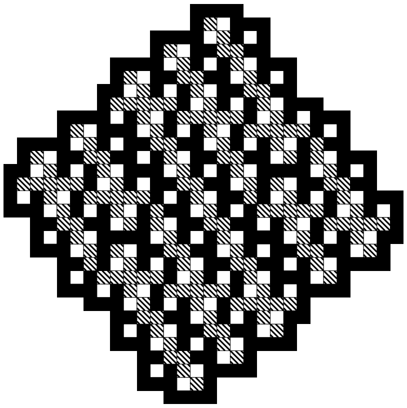
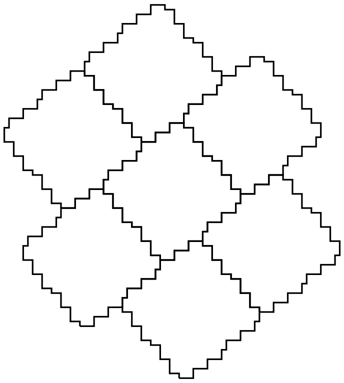

| | | |
|---|---|---|
| $(481, 241 + 418i)$ | | |
| $(192, 97 + 168i)$ | $23 + 12i$ | $11 + 7i$ |
| $(1, 1)$ | $-19 + 11i$ | $-11i$ |
| $(64, 31 + 56i)$ | $-4 - 23i$ | $-11 + 4i$ |
| $(33, 17 + 30i)$ | | |

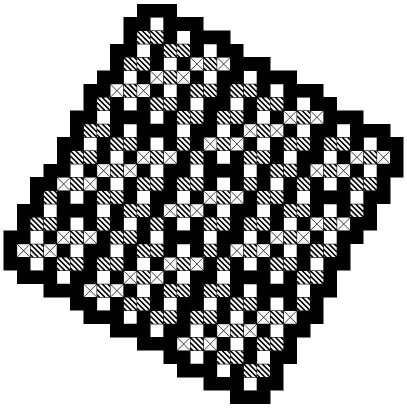
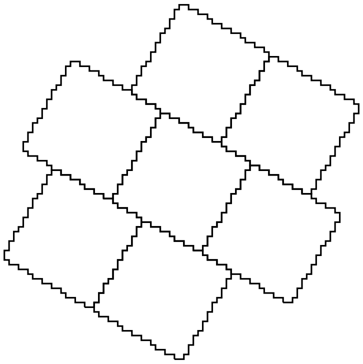

| | | |
|---|---|---|
| $(481, 241 + 470i)$ | | |
| $(321, 161 + 312i)$ | $-21 + 19i$ | $4 - 15i$ |
| $(4, 1 + 4i)$ | $-1 - 22i$ | $-11 + 5i$ |
| $(12, 7 + 12i)$ | $22 + 3i$ | $7 + 10i$ |
| $(193, 97 + 186i)$ | | |

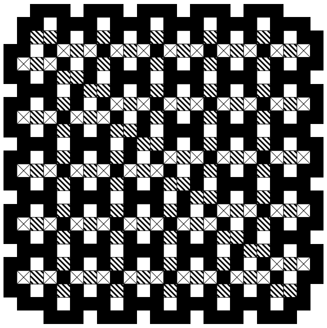
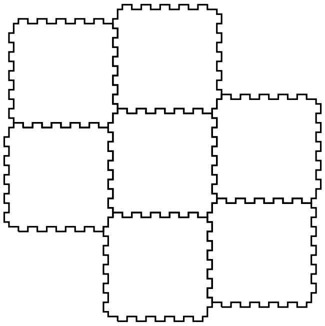

| | | |
|---|---|---|
| $(484, 1 + 44i)$ | | |
| $(441, 1 + 42i)$ | $22 + 21i$ | $1 + 1i$ |
| $(1, 1)$ | $-22 + 1i$ | $-1i$ |
| $(0, -1)$ | $-22i$ | $-1$ |
| $(400, 1 + 40i)$ | | |

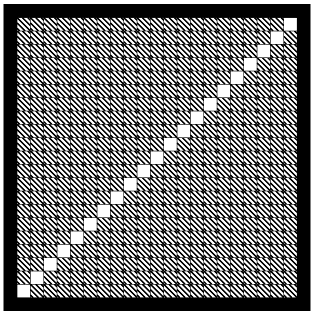
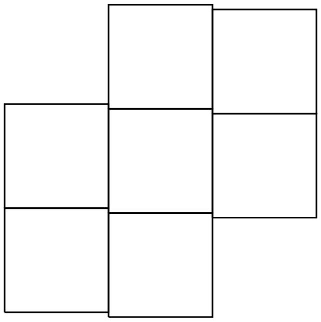

| | | |
|---|---|---|
| $(484, 1 + 132i)$ | | |
| $(225, 1 + 60i)$ | $-22 + 15i$ | $2 - 3i$ |
| $(0, -1)$ | $-22i$ | $-3$ |
| $(49, 1 + 14i)$ | $22 + 7i$ | $1 + 3i$ |
| $(64, 1 + 16i)$ | | |

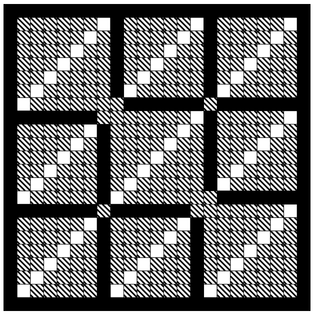
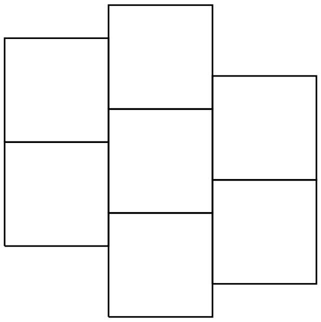

| | | |
|---|---|---|
| $(484, 1 + 220i)$ | | |
| $(169, 1 + 78i)$ | $22 + 13i$ | $3 + 5i$ |
| $(81, 1 + 36i)$ | $-22 + 9i$ | $2 - 5i$ |
| $(0, -1)$ | $-22i$ | $-5$ |
| $(16, 1 + 8i)$ | | |

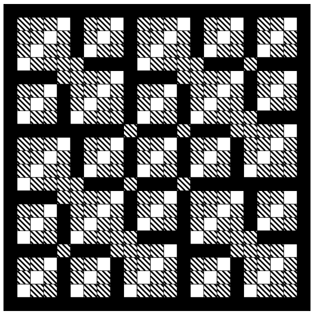
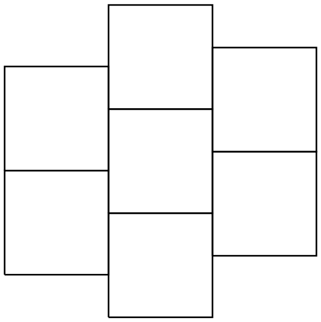

| | | |
|---|---|---|
| $(484, 1+308i)$ | | |
| $(361, 1+228i)$ | $-22+19i$ | $6-7i$ |
| $(0, -1)$ | $-22i$ | $-7$ |
| $(9, 1+6i)$ | $22+3i$ | $1+7i$ |
| $(256, 1+160i)$ | | |

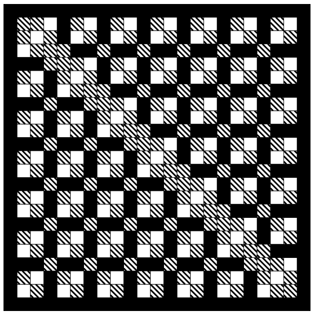
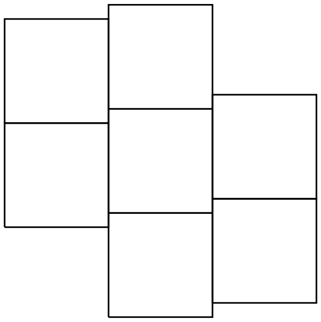

| | | |
|---|---|---|
| $(484, 1+396i)$ | | |
| $(289, 1+238i)$ | $22+17i$ | $7+9i$ |
| $(25, 1+20i)$ | $-22+5i$ | $2-9i$ |
| $(0, -1)$ | $-22i$ | $-9$ |
| $(144, 1+120i)$ | | |

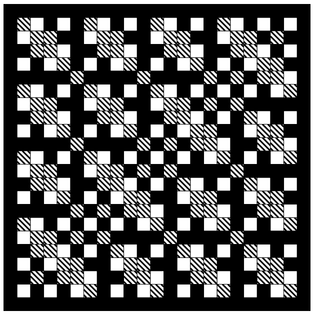
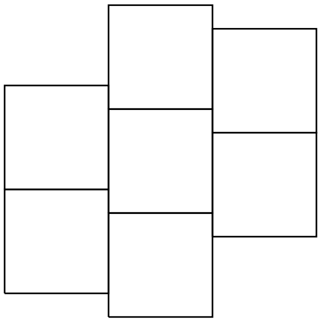

| | | |
|---|---|---|
| $(484, 391+476i)$ | | |
| $(201, 161+198i)$ | $-3-26i$ | $-14+9i$ |
| $(60, 49+60i)$ | $20+12i$ | $14+5i$ |
| $(1, 1)$ | $-17+14i$ | $-14i$ |
| $(40, 31+40i)$ | | |

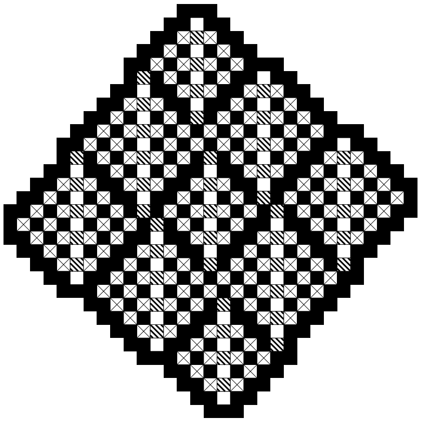
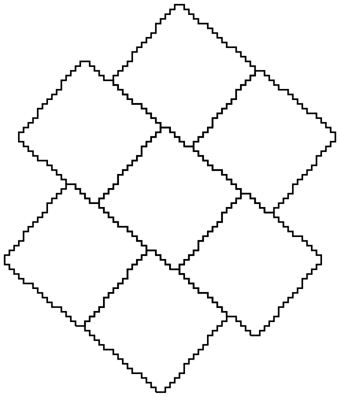

| | | |
|---|---|---|
| $(489, 17+216i)$ | | |
| $(244, 7+108i)$ | $-2-27i$ | $-6$ |
| $(16, 1+8i)$ | $19+12i$ | $3+4i$ |
| $(25, 1+10i)$ | $-17+15i$ | $3-4i$ |
| $(81, 1+36i)$ | | |

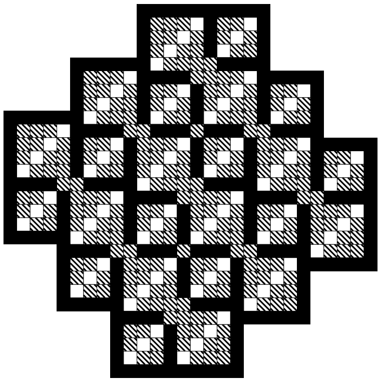
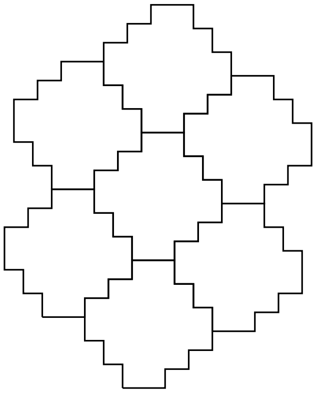

| | | |
|---|---|---|
| $(489, 161 + 372i)$ | | |
| $(145, 49 + 110i)$ | $-25 + 3i$ | $-3 - 10i$ |
| $(96, 31 + 72i)$ | $12 - 21i$ | $-6 + 8i$ |
| $(4, 1 + 4i)$ | $13 + 18i$ | $9 + 2i$ |
| $(1, 1)$ | | |

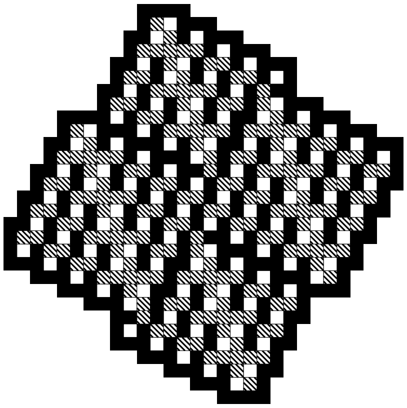

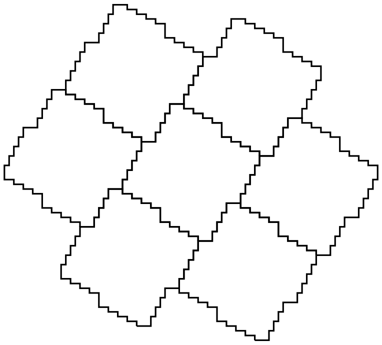

| | | |
|---|---|---|
| $(489, 241 + 456i)$ | | |
| $(256, 127 + 240i)$ | $24 + 13i$ | $12 + 8i$ |
| $(33, 17 + 30i)$ | $-21 + 9i$ | $-1 - 12i$ |
| $(4, 1 + 4i)$ | $-3 - 22i$ | $-11 + 4i$ |
| $(97, 49 + 92i)$ | | |

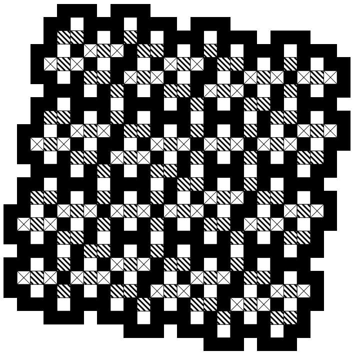

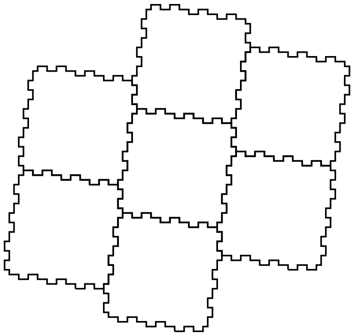

| | | |
|---|---|---|
| $(492, 17 + 132i)$ | | |
| $(228, 7 + 60i)$ | $12 - 24i$ | $-3 + 2i$ |
| $(49, 1 + 14i)$ | $10 + 21i$ | $3 + 1i$ |
| $(1, 1)$ | $-22 + 3i$ | $-3i$ |
| $(64, 1 + 16i)$ | | |

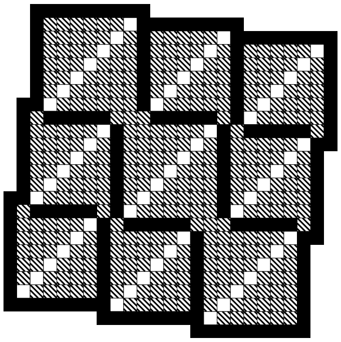

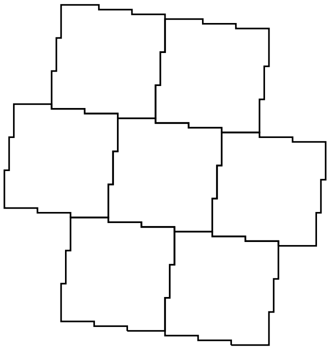

| | | |
|---|---|---|
| $(492, 337 + 468i)$ | | |
| $(184, 127 + 176i)$ | $24 + 10i$ | $13 + 8i$ |
| $(1, 1)$ | $-18 + 13i$ | $-13i$ |
| $(73, 49 + 70i)$ | $-6 - 23i$ | $-13 + 5i$ |
| $(24, 17 + 24i)$ | | |

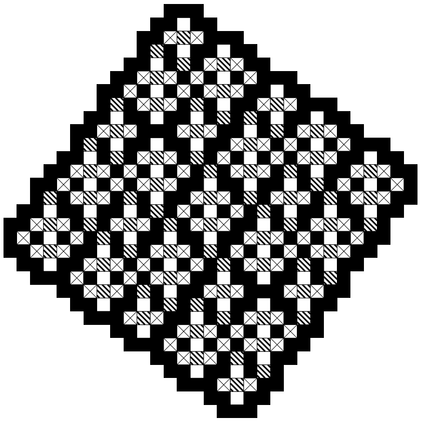

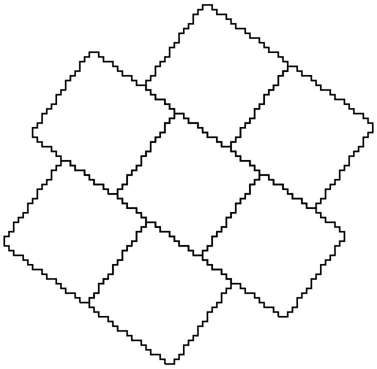

| | | |
|---|---|---|
| $(496, 31 + 216i)$ | | |
| $(249, 17 + 108i)$ | $-27 + 4i$ | $-6i$ |
| $(25, 1 + 10i)$ | $11 - 20i$ | $-4 + 3i$ |
| $(16, 1 + 8i)$ | $16 + 16i$ | $4 + 3i$ |
| $(84, 7 + 36i)$ | | |

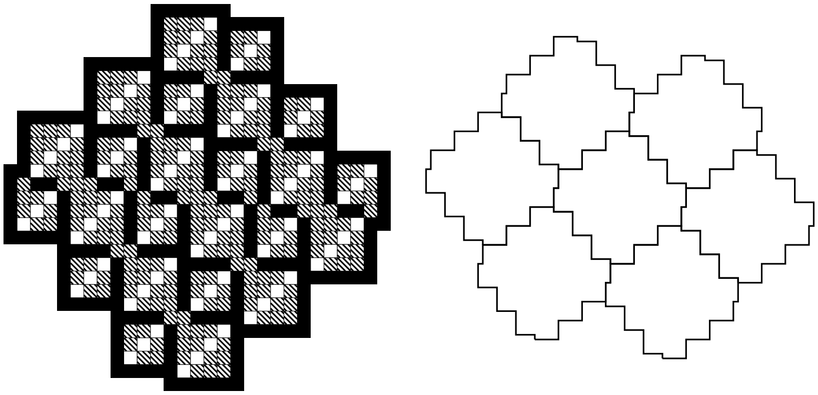

| | | |
|---|---|---|
| $(496, 31 + 280i)$ | | |
| $(297, 17 + 168i)$ | $-3 - 28i$ | $-8$ |
| $(9, 1 + 6i)$ | $19 + 12i$ | $4 + 5i$ |
| $(16, 1 + 8i)$ | $-16 + 16i$ | $4 - 5i$ |
| $(148, 7 + 84i)$ | | |

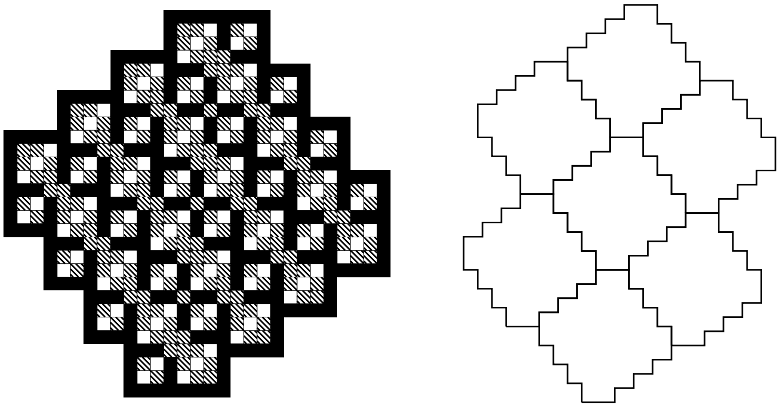

| | | |
|---|---|---|
| $(496, 97 + 368i)$ | | |
| $(160, 31 + 120i)$ | $16 + 20i$ | $9 + 4i$ |
| $(81, 17 + 60i)$ | $-24 + 1i$ | $-2 - 9i$ |
| $(9, 1 + 6i)$ | $8 - 21i$ | $-7 + 5i$ |
| $(4, 1 + 4i)$ | | |

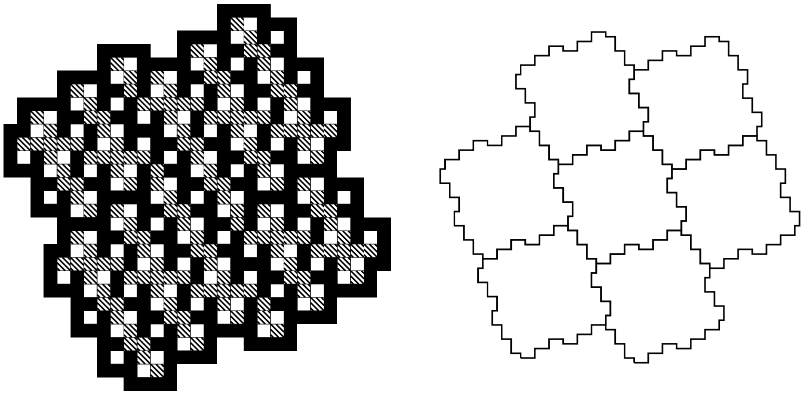

Supplement: Supplementary file 1 [file bigappendix.pdf]
